# Supplementary material for: Model-free Test Time Adaptation for Out-Of-Distribution Detection
Source: arXiv:2311.16420 source file (2023-11-28)
Supplement: Supplementary file 1 [file appendix_holder.tex]

\section{Proof of theoretical statement}

\subsection{Non-parametric reduce target-source domain divergence}
To complete the proofs, we begin by introducing some necessary definitions and assumptions. 
\begin{definition}
(\textbf{Wasserstein-distance and the dual form} ~\cite{arjovsky2017wasserstein}). The $\rho$-th Wasserstein distance between two distributions $\mathbbm{D}_S, \mathbbm{D}_U$ is defined as
\begin{equation}
\mathcal{W}_\rho(\mathbbm{D}_S,\mathbbm{D}_U)=\left(\inf_{\gamma\in \Pi[\mathbbm{D}_S,\mathbbm{D}_U]} \iint d({x_s},{x_u})^\rho  d\gamma({x_s},{x_u})\right)^{1/\rho}
\label{eq:wd}
\end{equation}
where $\Pi[\mathbbm{D}_S,\mathbbm{D}_U]$ is the set of all joint distribution on $\mathcal{X}\times\mathcal{X}$ with marginals $\mathbbm{D}_S$ and $\mathbbm{D}_U$ and $d(x_s,x_u)$ is a distance function for two instances $x_s,x_u$.

Wasserstein distance can get intuition from the optimal transport problem, where $d(x_s,x_u)^\rho$ is the unit cost for transporting a unit of material from $x_s\in \mathbbm{D}_S$ to $x_u\in \mathbbm{D}_U$ and $\gamma(x_s,x_u)$ is the transport policy which satisfies the marginal constraint. According to the Kantorovich-Rubinstein theorem, the dual representation of the first Wasserstein distance (Earth-Mover distance) can be written as
\begin{equation}
\mathcal{W}_1(\mathbbm{D}_S,\mathbbm{D}_U)=\sup_{\parallel f\parallel_L\leq 1} \mathbb{E}_{x_s\in \mathbbm{D}_S}[f(x_s)]-\mathbb{E}_{x_u\in \mathbbm{D}_U}[f(x_u)],
\end{equation}
where $\parallel f\parallel_L=\sup|f(x_s)-f(x_u)|/d(x_s,x_u)$ is the Lipschitz semi-norm. 
\label{define1}
\end{definition}

We first use the domain adaptation result, Theorem 1 in~\cite{shen2018wasserstein} that considers the Wasserstein distance. On this basis, we can clearly show the effect of \knn on the domain divergence. In this paper, we use $\mathcal{W}_1(\mathbbm{D}_S,\mathbbm{D}_U)$ as default and ignore subscript 1. For completeness, we present the Theorem 1 in~\cite{shen2018wasserstein} as follow:

\begin{prop}
(Theorem 1 in~\cite{shen2018wasserstein}) Given two domain distributions $\mathbbm{D}_S,\mathbbm{D}_U$, denote $f^*=\arg\min_{f\in\mathcal{H}}(\epsilon_U(f)+\epsilon_S(f))$ and $\kappa=\epsilon_U(f^*)+\epsilon_S(f^*)$. Assume all hypotheses $h$ are $L$-Lipschitz continuous, the risk of hypothesis $\hat{f}$ on the unseen target domain is then bounded by
\begin{equation}
    \epsilon_U(\hat{f})\leq \kappa+\epsilon_S(\hat{f})+2L\mathcal{W}(\mathbbm{D}_S,\mathbbm{D}_U).
    \label{lemma:bound}
\end{equation}
\label{prop:wass}
\end{prop}

Intuitively, by using the non-parametric classifier, during inference, a large number of samples in source domains that do not similar to the target samples are ignored, and thus the domain divergence will be reduced. That is, the source distribution $\mathbbm{D}_S$ is replaced by $\Omega:=\bigcup_{x\in \mathbbm{D}_U} \mathcal{B}(x,r)$, where $\mathcal{B}(x,r)=\{x':\parallel x'-x\parallel\leq r\}$ denotes a ball centered on $x$ with radius $r$, and With a small $r$, $\Omega$ is intuitively close to $\mathbbm{D}_U$ because these dissimilar data points are ignored and the selected source data are all close to the target data. Informally, according to \myref{eq:wd}, we have $\mathcal{W}(\Omega,\mathbbm{D}_U)=\inf_{\gamma\in \Pi[\Omega,\mathbbm{D}_U]} \iint \parallel {x_s}-{x_u}\parallel  d\gamma({x_s},{x_u})$, where for each $x_s\in\Omega$, we can find at least one $x_u\in \mathbbm{D}_U$ such that $\parallel x_s-x_u\parallel\leq r$, the overall distance will then be bounded by $r$. If $r$ is small enough, $\mathcal{W}(\mathbbm{D}_S,\mathbbm{D}_U)$ in Proposition~\ref{prop:wass} is largely reduced. Specifically, we can choose a density function $\gamma^*$ where $\gamma^*(x_s,x_u)>0$ only if $x_s\in B(x_u,r)$ otherwise 0, then we have

\begin{equation}
\mathcal{W}(\Omega,\mathbbm{D}_U)=\inf_{\gamma\in \Pi[\Omega,\mathbbm{D}_U]} \iint \parallel {x_s}-{x_u}\parallel  d\gamma({x_s},{x_u})\leq  \iint \parallel {x_s}-{x_u}\parallel \gamma^*({x_s},{x_u})  d x_sx_u\leq r
\end{equation}

Although a small $r$ will reduce the generalization bound, there is no guarantee that each data $x_u\in \mathbbm{D}_U$ can find a neighbor $B(x,r)$ with $|B(x,r)|>0$. To this end, we theoretically discuss the choice of $r$ and show \textit{given a choice radius $r$, what probability that the set of neighbors $B(x,r)$ of each $x\in \mathbbm{D}_U$ is not measuring zero}?

We denote $k$ is the number of neighbors that we prefer to choose, namely the parameter for the KNN classifier, $n_s$ is the total number of data in ${D}_S$. With the strong density assumption, for any $x_u\in \mathbbm{D}_U, r<r_\mu$, according to Assumption~\ref{assump1}, we have

\begin{equation}
\mathbbm{D}_S(x_s\in B(x_u,r))=\int_{B(x_u,r)\cap \mathbbm{D}_S} \frac{d \mathbbm{D}_S}{d\lambda}(x_s)dx_s\geq \mu_-\lambda(B(x_u,r)\cap \mathbbm{D}_S)\geq c_\mu\mu_-\pi_dr^d,
\label{equ:a}
\end{equation}

where $\pi_d=\lambda(B(0,1))$ is the volume of the $d$ dimension unit ball and $\lambda$ is the Lebesgue measure of a set in a Euclidean space. Set $r_0=(\frac{2k}{c_\mu\mu_-\pi_dn_s})^{1/d}$, with a additional assumption that $\frac{k}{n_s}<\frac{c_\mu\mu_-\pi_dr_\mu^d}{2}$\footnote{The assumption is rational because, $n_s\gg k$ in general.}, we have $r_0<r_\mu$. Then for any $x_u\in \mathbbm{D}_U$, according to \myref{equ:a}, we have
\begin{equation}
    \mathbbm{D}_S(x_s\in B(x_u,r_0)) \geq  c_\mu\mu_-\pi_dr_0^d >\frac{2k}{n_s}
\end{equation}
Denote $\mathbb{I}$ an indicator function and then $\mathbb{I}(x_s\in B(x_u,r_0))$  are independent and identically Bernuoli variables, which mean is $\mathbbm{D}_S(x_s\in B(x_u,r_0))$. Let $S_n(x_u)=\sum_{i=1}^{n_s}\mathbb{I}(x_s\in B(x_u,r_0))$ denote the number of data $x_s\in \mathbbm{D}_S$ that fall into $B(x,r_0)$, then $S_n(x_u)$ follows the Binomial distribution. Let $W\sim Binomial(n_s,\frac{2k}{n_s})$, according to the Chernoff inequality~\cite{chernoff1981note,chung2006concentration},

\begin{equation}
    P(S_n(x_u)<k)\leq P(W<k)= P(W-\mathbb{E}[W]<-k)\leq \exp(-k^2/2\mathbb{E}[W])=\exp(-k/4),
\end{equation}

where the second inequality is because $S_n(x)$ has a larger mean than $W$. We can see the probability that $S_n(x)<k$ is small for any $x_u\in \mathbbm{D}_U$, especially when $k$ is large. Denoting $x_s^{(i)}$ the $i-$th nearest data to $x_u$ among $B(x_u,r_0)$, we have for any $x_u\in \mathbbm{D}_U$

\begin{equation}
P(\parallel x_s^{(k)}-x_u \parallel\leq r_0)= P(S_n(x)\geq k)\geq 1-\exp(-k/4)
\label{bound:x_diff}
\end{equation}
{\color{red}\textbf{ the union bound is unreasonable, considering distribution, there are infinite instances.}

Now we can conclude that we have $\parallel x_s^{(k)}-x_u \parallel\leq (\frac{2k}{c_\mu\mu_-\pi_dn_s})^{1/d}$ with probability at least $1-\exp(-k/4)$. Finally, we can get a union bound
\begin{equation}
\bigcap_{x_u\in \mathbbm{D}_U} P(\parallel x_s^{(k)}-x_u \parallel\leq r_0)=\bigcap_{x_u\in \mathbbm{D}_U} P(S_n(x)\geq k)=1-\bigcup_{x_u\in \mathbbm{D}_U}P(S_n(x)< k) \geq 1-n\exp(-k/4)
\end{equation}
}

\subsection{Analysis of the excess error upper-bound under covariate-shift}
\textbf{Under the covariate-shift setting}, we have $\eta_U=\eta_S=\eta$ for source and target domains. We denote the KNN classifier with $k$ nearest neighbors as $\hat{f}_k=\mathbb{I}\{\hat{\eta}_k\geq \frac{1}{2}\}$. Because we focus on the binary classification setting, then $\hat{f}_k(x_u)\neq f_U^*(x_u)$ implies that $\left| \hat{\eta}_k(x_u) -\eta(x_u)\right|\geq \left|\eta(x_u)-\frac{1}{2}\right|$. In this way, we can build the connection between the excess error and the regress error:
\begin{equation}
    \mathcal{E}_U(\hat{f})=2\mathbb{E}_{x_u\sim \mathbbm{D}_U}\left[\left|\eta(x_u)-\frac{1}{2}\right|\mathbb{I}\left\{\left| \hat{\eta}_k(x_u) -\eta(x_u)\right|\geq \left|\eta(x_u)-\frac{1}{2}\right|\right\}\right]
\end{equation}

Let $Z=\left|\eta(x_u)-\frac{1}{2}\right|$, if we can bound $\sup_{x_u} \left| \hat{\eta}_k(x_u) -\eta(x_u) \right|\leq t$, then by the marginal assumption in Definition~\ref{define_noise} and the fact that 
\begin{equation}
    \mathbb{E}\left[Z\cdot \mathbb{I}\{Z\leq t\}\right]\leq tP(Z\leq t),
\label{equ:indcator}
\end{equation}
we have $ \mathcal{E}_U(\hat{f})\leq C_\beta t^{\beta+1}$. To bound $\left| \hat{\eta}_k(x_u) -\eta(x_u) \right|$, we denote $(x_s^{(i)},y_s^{(i)})$ as the $i-$th nearest data and the corresponding labels to $x_u$ in $B(x_u,r_0)$. The KNN classification result will be $\hat{\eta}(x_u)=\sum_{i=1}^k w_i y_s^{(i)}$, where $w_i$ is the weight for the $i$ -th nearest neighbor, and $\sum_{i=1}^k w_i=1$. In this work, we use the cosine similarity as the weight, where the distance-weighted KNN is shown able to reduce the misclassification error~\cite{dudani1976distance}. However, for brevity of the proof, we assume $w_i=\frac{1}{k},\forall i\in[1,...,k]$, namely all nearest data labels are uniformly mixed. Based on the assumptions and notions above, we have for any $x_u\in \mathbbm{D}_U$

\begin{equation}
\begin{aligned}
\left|\hat{\eta}_k(x_u) -\eta(x_u) \right |&=\left| \frac{1}{k}\sum_{i=1}^k y_s^{(i)}-\eta(x_u)  \right|\\
& \leq \left|\frac{1}{k}\sum_{i=1}^k y_s^{(i)}-\frac{1}{k}\sum_{i=1}^k\eta\left(x_s^{(i)}\right)\right|+\left| \frac{1}{k}\sum_{i=1}^k\eta\left(x_s^{(i)}\right)-\eta(x_u)  \right|\\
&\leq \underbrace{\frac{1}{k}\left| \sum_{i=1}^k y_s^{(i)}-\sum_{i=1}^k \eta\left(x_s^{(i)}\right)\right|}_{\rm \circled{\rm 1}}+\underbrace{\frac{1}{k}\sum_{i=1}^k\left| \eta\left(x_s^{(i)}\right)-\eta(x_u)  \right|}_{\rm \circled{\rm 2}},
\end{aligned}
\label{equ:bound_cova}
\end{equation}
where ${\rm \circled{\rm 2}}$ is easy to bound. According to the assumption that $\eta_U$ is $(\alpha, C_\alpha)-H\ddot{o}lder$, we have
\begin{equation}
\sum_{i=1}^k\frac{1}{k}\left| \eta\left(x_s^{(i)}\right)-\eta(x_u)  \right|\leq  \sum_{i=1}^k\frac{1}{k} C_\alpha \cdot \parallel x_s^{(i)}- x_u \parallel^\alpha \leq C_\alpha \cdot \parallel x_s^{(k)}- x_u \parallel^{\alpha}
\label{equ:19}
\end{equation}
According to \myref{bound:x_diff}, with probability at least $1-\exp(-k/4)$, ${\rm \circled{\rm 2}}\leq C_\alpha\left(\frac{2k}{c_\mu\mu_-\pi_dn_s}\right)^{1/d}$. Note that $E_{Y|X}[y_s^{(i)}]=\eta(x_s^{(i)})$, we then use the Hoeffding inequality to get the upperbound of ${\rm \circled{\rm 1}}$
\begin{equation}
P_{X,Y}\left(\frac{1}{k}\left|\sum_{i=1}^k y_s^{(i)}-\sum_{i=1}^k\eta\left(x_s^{(i)}\right)\right|>\epsilon\right)=\mathbb{E}_X\left[P_{Y|X}\left(\frac{1}{k}\left|\sum_{i=1}^k y_s^{(i)}-\sum_{i=1}^k\eta\left(x_s^{(i)}\right)\right|>\epsilon\right)\right]\leq 2\exp(-2k\epsilon^2)
\label{equ:21}
\end{equation}
% Set $\epsilon=(1/k)^{1/4}$, we have, with probability, at least $1-\exp(-k/4)$, ${\rm \circled{\rm 1}}\leq (1/k)^{1/4}$, ${\rm \circled{\rm 2}}\leq C_\alpha\left(\frac{2k}{c_\mu\mu_-\pi_dn_s}\right)^{1/d}$, and then $\left|\hat{\eta}_k(x_u) -\eta(x_u) \right |\leq (1/k)^{1/4}+C_\alpha\left(\frac{2k}{c_\mu\mu_-\pi_dn_s}\right)^{1/d}$. According to \myref{bound:x_diff} and \myref{equ:indcator}, the excess error is bounded by
Set $\epsilon=(1/k)^{1/4}$, we have, with probability, at least $1-2\exp(-2\sqrt{k})$, ${\rm \circled{\rm 1}}\leq(1/k)^{1/4}$, ${\rm \circled{\rm 2}}\leq C_\alpha\left(\frac{2k}{c_\mu\mu_-\pi_dn_s}\right)^{1/d}$, and then $\left|\hat{\eta}_k(x_u) -\eta(x_u) \right |\leq (1/k)^{1/4}+C_\alpha\left(\frac{2k}{c_\mu\mu_-\pi_dn_s}\right)^{1/d}$. According to \myref{bound:x_diff} and \myref{equ:indcator}, the excess error is bounded by

% \begin{equation} # a compelex episilon
% \mathcal{E}_U(\hat{f})\leq 2C_\beta\left( \left(\frac{\ln 2}{2k}+\frac{1}{8}\right)^{1/4}+  C_\alpha\left(\frac{2k}{c_\mu\mu_-\pi_dn_s}\right)^{\alpha /{d}}\right)^{{1+\beta}}\approx \left(C_1\left(\frac{1}{k}\right)^{1/4}+C_2  \left(\frac{k}{c_\mu n_s}\right)^{\alpha /{d}} \right)^{{1+\beta}},
% \label{bound:22}
% \end{equation}
\begin{equation}
\mathcal{E}_U(\hat{f})\leq 2C_\beta\left( \left(\frac{1}{k}\right)^{1/4}+  C_\alpha\left(\frac{2k}{c_\mu\mu_-\pi_dn_s}\right)^{\alpha /{d}}\right)^{{1+\beta}}\approx \left(\left(\frac{1}{k}\right)^{1/4}+C_1  \left(\frac{k}{c_\mu n_s}\right)^{\alpha /{d}} \right)^{{1+\beta}},
\label{bound:22}
\end{equation}
where $C_1$ is a newly introduced constant. There is a clear tradeoff between the upper bound of ${\rm \circled{\rm 1}}$ and ${\rm \circled{\rm 2}}$ with respect to the value of $k$. A small $k$ will reduce the representation difference in ${\rm \circled{\rm 2}}$, extremely when $k=1$, only the nearest sample to $x_u$ will be chosen. However, when $k$ is small, there is no guarantee that the nearest selected data will have a confident prediction. Specifically, a smaller ${\rm \circled{\rm 1}}$ indicates that the selected $k$ nearest data samples are representative enough and have confident prediction results. According to the assumption~\ref{assump2}, we have with probability at least $\min\{ 1-\exp(-n_s^\delta/4),  1-2\exp(-2\sqrt{n_s^\delta})\}$, 

\begin{equation}
\mathcal{E}_U(\hat{f})\leq  \left(\left(\frac{1}{n_s}\right)^{\delta/4}+C_1  \left(\frac{1}{c_\mu n_s^{1-\delta}}\right)^{\alpha /{d}} \right)^{{1+\beta}},
\end{equation}

\subsection{Analysis of the excess error upper-bound under posterior-shift settings}
\textbf{Under the posterior-shift setting}, the support of $\mathbbm{D}_S$ and $\mathbbm{D}_U$ are the same, i.e., $\text{Supp}(\mathbbm{D}_S)=\text{Supp}(\mathbbm{D}_U)=\Omega$. The regression functions $\eta_U$ and $\eta_S$ are different. Then we have
\begin{equation}
\begin{aligned}
\left|\hat{\eta}_k(x_u) -\eta_U(x_u) \right |&=\left| \frac{1}{k}\sum_{i=1}^k y_s^{(i)}-\eta_U(x_u) \right|\\
&\leq \left|\frac{1}{k}\sum_{i=1}^k y_s^{(i)}-\frac{1}{k}\sum_{i=1}^k\eta_S\left(x_s^{(i)}\right)\right|+\left| \frac{1}{k}\sum_{i=1}^k\eta_S\left(x_s^{(i)}\right)-\eta_U(x_u)  \right|\\
&=\frac{1}{k}\left| \sum_{i=1}^k y_s^{(i)}-\sum_{i=1}^k\eta\left(x_s^{(i)}\right)\right|+\frac{1}{k}\sum_{i=1}^k\left| \eta_S\left(x_s^{(i)}\right)-\eta_U(x_u)  \right|\\
&=\frac{1}{k} \left| \sum_{i=1}^ky_s^{(i)}-\sum_{i=1}^k\eta\left(x_s^{(i)}\right)\right|+\frac{1}{k}\sum_{i=1}^k\left| \eta_S\left(x_s^{(i)}\right)-\eta_S(x_u)+\eta_S(x_u)-\eta_U(x_u)  \right|\\
&\leq\frac{1}{k} \left| \sum_{i=1}^ky_s^{(i)}-\sum_{i=1}^k\eta\left(x_s^{(i)}\right)\right|+\frac{1}{k}\sum_{i=1}^k\left| \eta_S\left(x_s^{(i)}\right)-\eta_S(x_u)\right|+ \underbrace{\left|\eta_S(x_u)-\eta_U(x_u)  \right|}_{\text{Adaptivity gap}}
% &\leq C_\alpha C_\delta \cdot \parallel x_s^{(k)}- x_u \parallel^{\alpha-\delta}+\left|\eta_S(x_u)-\eta_U(x_u)  \right|\\
\end{aligned}
\label{equ:bound_post}
\end{equation}
Compared to \myref{equ:bound_cova}, \myref{equ:bound_post} has an additional term $\left|\eta_S(x_u)-\eta_U(x_u)  \right|$ (the adaptivity gap~\cite{zhang2022domain}), which measure the difference of two regression functions directly. Although previous work has similar definition, for example, the regression functions difference defined in~\cite{zhao2019learning}: $\min\{{\mathbb{E}_{\mathbbm{D}_S}[|\eta_S-\eta_U|]},\mathbb{E}_{\mathbbm{D}_U}[|\eta_S-\eta_U|]\}$, which care about ``how $\eta_U$ performs on source data''. In comparison, our definition is more similar to~\cite{zhang2022domain}, which only focuses on the regression difference when evaluated on examples from the target domain and shown to be more practical and intuitive~\cite{kpotufe2018marginal,zhang2022domain}.

% The last line uses the inequality in \myref{equ:bound_cova}. According to the definition of relative signal exponent, we have
% \begin{equation}
% \begin{aligned}
%     \left|\eta_S(x_u)-\eta_U(x_u)  \right|&=\left|\eta_S(x_u)-\frac{1}{2}+\frac{1}{2}-\eta_U(x_u)  \right| \\
%     &\leq \left|\eta_S(x_u)-\frac{1}{2}\right|+\left|\eta_U(x_u)-\frac{1}{2} \right|\\
%     &\leq \left(\frac{1}{C_\gamma}\left|\eta_U(x_u)-\frac{1}{2} \right|\right)^{1/\gamma}+\left|\eta_U(x_u)-\frac{1}{2} \right|
% \end{aligned}
% \end{equation}
We assume that $|\eta_S-\eta_U|$ is upper bounded by some constant $C_{ada}$, namely $\sup_{x_u\in \mathbbm{D}_U} |\eta_S(x_u)-\eta_U(x_u)|\leq C_{ada}$, under the posterior-shift setting, we have
\begin{equation}
\mathcal{E}_U(\hat{f})\leq \left(\left(\frac{1}{k}\right)^{1/4}+C_1  \left(\frac{k}{c_\mu n_s}\right)^{\alpha /{d}} +C_{ada} \right)^{{1+\beta}}
\end{equation}
% \begin{equation}
% \begin{aligned}
% &\mathcal{E}_U(\hat{f})=2\mathbb{E}_{x\sim \mathbbm{D}_U}\left[\left|\eta_U(x)-\frac{1}{2}\right|\mathbb{I}\left\{\left|\eta_U(x)-\frac{1}{2}\right|\leq \left| \hat{\eta}_k(x) -\eta_U(x)\right| \right\}\right]\\
% &\leq 2\mathbb{E}_{x\sim \mathbbm{D}_U}\left[\left|\eta_U(x)-\frac{1}{2}\right|\mathbb{I}\left\{\left|\eta_U(x)-\frac{1}{2}\right|\leq  C_\alpha C_\delta \cdot \parallel x_s^{(k)}- x \parallel^{\alpha-\delta}+ \left(\frac{1}{C_\gamma}\left|\eta_U(x)-\frac{1}{2} \right|\right)^{1/\gamma}+\left|\eta_U(x)-\frac{1}{2} \right|\right\}\right]\\
% \end{aligned}
% \end{equation}

According to assumption~\ref{assump2}, we have with probability at least $\min\{ 1-\exp(-n_s^\delta/4),  1-2\exp(-2\sqrt{n_s^\delta})\}$, 
\begin{equation}
\mathcal{E}_U(\hat{f})\leq  \left(\left(\frac{1}{n_s}\right)^{\delta/4}+C_1  \left(\frac{1}{c_\mu n_s^{1-\delta}}\right)^{\alpha /{d}} +C_{ada}\right)^{{1+\beta}}
\end{equation}
\subsection{Effect of utilizing online target samples}

Despite the assumptions and notions mentioned above, to study the effect of target data, we denote $\{x_s^{(i)},y_s^{(i)}\}_{i=1}^{k_s}+\{x_u^{(i)},y_u^{(i)}\}_{i=1}^{k_u}$ as the nearest data and the corresponding labels to $x_u$ in $B(x_u,r_0)$, where $k_s+k_u=k$ and $y_u^{(i)}$ is the pseudo-label of $x_u^{(i)}$, that is, $y_u^{(i)}=\mathbb{I}\{\hat{\eta}_k(x_u^{(i)})\geq 1/2\}$. The KNN classification result will be $\hat{\eta}_k(x_u)=\frac{1}{k}\sum_{i=1}^{k_s} y_s^{(i)}+\frac{1}{k}\sum_{i=1}^{k_u} y_u^{(i)}$. We have the following.

\begin{equation}
\begin{aligned}
\left|\hat{\eta}_k(x_u) -\eta(x_u) \right |&=\left| \frac{1}{k}\sum_{i=1}^{k_s} y_s^{(i)}-\frac{1}{k}\sum_{i=1}^{k_s}\eta(x_u) +\frac{1}{k}\sum_{i=1}^{k_u} y_u^{(i)}-\frac{1}{k}\sum_{i=1}^{k_u}\eta(x_u)  \right|\\
& \leq \left|\frac{1}{k}\sum_{i=1}^{k_s} y_s^{(i)}-\frac{1}{k}\sum_{i=1}^{k_s} \eta\left(x_s^{(i)}\right)\right|+\left| \frac{1}{k}\sum_{i=1}^{k_s} \eta\left(x_s^{(i)}\right)-\frac{k_s}{k}\eta(x_u)  \right|\\
&\quad\quad\quad +\left|\frac{1}{k}\sum_{i=1}^{k_u} y_u^{(i)}-\frac{1}{k}\sum_{i=1}^{k_u} \eta\left(x_u^{(i)}\right)\right|+\left| \frac{1}{k}\sum_{i=1}^{k_u} \eta\left(x_u^{(i)}\right)-\frac{k_u}{k}\eta(x_u)  \right|\\
% &\leq \underbrace{\frac{1}{k}\left|\sum_{i=1}^{k_s} y_s^{(i)}-\sum_{i=1}^{k_s}\eta\left(x_s^{(i)}\right)\right|}_{\rm \circled{\rm 1}}+\underbrace{\frac{1}{k}\sum_{i=1}^{k_s}\left| \eta\left(x_s^{(i)}\right)-\eta(x_u)  \right|}_{\rm \circled{\rm 2}}\\
% &\quad\quad\quad + \underbrace{\frac{1}{k}\left| \sum_{i=1}^{k_u}y_u^{(i)}-\sum_{i=1}^{k_u}\eta\left(x_u^{(i)}\right)\right|}_{\rm \circled{\rm 3}}+\underbrace{\frac{1}{k}\sum_{i=1}^{k_u}\left| \eta\left(x_u^{(i)}\right)-\eta(x_u)  \right|}_{\rm \circled{}}
&\leq \underbrace{\frac{1}{k}\left|\sum_{i=1}^{k_s} y_s^{(i)}+\sum_{i=1}^{k_u}y_u^{(i)}-\sum_{i=1}^{k_s}\eta\left(x_s^{(i)}\right)-\sum_{i=1}^{k_u}\eta\left(x_u^{(i)}\right)\right|}_{\rm \circled{\rm 1}}+\underbrace{\frac{1}{k}\sum_{i=1}^{k_s}\left| \eta\left(x_s^{(i)}\right)-\eta(x_u)  \right|}_{\rm \circled{\rm 2}}\\
&\quad\quad\quad+\underbrace{\frac{1}{k}\sum_{i=1}^{k_u}\left| \eta\left(x_u^{(i)}\right)-\eta(x_u)  \right|}_{\rm \circled{\rm 3}}
\end{aligned}
\end{equation}
Although the true labels of target samples are unknown, we store the target sample into the KNN query set only when its prediction confidence is large enough. Therefore, it is natural to assume that $\mathbb{E}_{Y|X}[y_u^{(i)}]=\eta(x_u^{(i)})$. According to \myref{equ:21}, we have
% \begin{equation}
% P_{X,Y}\left(\frac{1}{k}\left|\sum_{i=1}^{k_s} y_s^{(i)}-\sum_{i=1}^{k_s}\eta\left(x_s^{(i)}\right)\right|>\epsilon\right)=\mathbb{E}_X\left[P_{Y|X}\left(\frac{1}{k}\left|\sum_{i=1}^{k_s} y_s^{(i)}-\sum_{i=1}^{k_s}\eta\left(x_s^{(i)}\right)\right|>\epsilon\right)\right]\leq 2\exp(\frac{-2k^2\epsilon^2}{k_s})
% \label{equ:27}
% \end{equation}
\begin{equation}
\begin{aligned}
&P_{X,Y}\left(\frac{1}{k}\left|\sum_{i=1}^{k_s} y_s^{(i)}+\sum_{i=1}^{k_u}y_u^{(i)}-\sum_{i=1}^{k_s}\eta\left(x_s^{(i)}\right)-\sum_{i=1}^{k_u}\eta\left(x_u^{(i)}\right)\right|\right)\\
&=\mathbb{E}_X\left[P_{Y|X}\left(\frac{1}{k}\left|\sum_{i=1}^{k_s} y_s^{(i)}+\sum_{i=1}^{k_u}y_u^{(i)}-\sum_{i=1}^{k_s}\eta\left(x_s^{(i)}\right)-\sum_{i=1}^{k_u}\eta\left(x_u^{(i)}\right)\right|
\right)\right]\leq 2\exp({-2k\epsilon^2})
\end{aligned}
\label{equ:27}
\end{equation}
% Set $\epsilon=\sqrt{\frac{k_s\ln 2}{2k^2}+\frac{k_s^2}{8k^2}}$, we have with probability at least $1-\exp(-k_s/4)$, ${\rm \circled{\rm 1}}\leq \sqrt{\frac{k_s\ln 2}{2k^2}+\frac{k_s}{8k}}$. Similarly we can get ${\rm \circled{\rm 3}}\leq \sqrt{\frac{k_u\ln 2}{2k^2}+\frac{k_u^2}{8k^2}}$ with probabilty at least $1-\exp(-k_u/4)$. According to \myref{equ:19}, we have
Set $\epsilon=(1/k)^{1/4}$, we have, with probability, at least $1-2\exp(-2\sqrt{k})$, ${\rm \circled{\rm 1}}\leq (1/k)^{1/4}$. Then, according to \myref{equ:19}, we have
\begin{equation}
{\rm \circled{\rm 2}}\leq \frac{k_s}{k} C_\alpha\left(\frac{2k_s}{c_\mu\mu_-\pi_dn_s}\right)^{\alpha/d}; {\rm \circled{\rm 3}}\leq \frac{k_u}{k} C_\alpha\left(\frac{2k_u}{c_\mu^*\mu_-\pi_dn_u}\right)^{\alpha/d}
\end{equation}
% Finally, we have that, with probability at least $1-\max\{\exp(-k_s/4),\exp(-k_u/4)\}$,  the excess error under the covariate shift setting can be bounded by
% \begin{equation}
% \begin{aligned}
% \mathcal{E}_U(\hat{f})&\leq 2C_\beta\left( 
% \sqrt{\frac{k_s\ln 2}{2k^2}+\frac{k_s^2}{8k^2}} + \sqrt{\frac{k_u\ln 2}{2k^2}+\frac{k_u^2}{8k^2}}
% + \frac{k_s}{k}C_\alpha\left(\frac{2k_s}{c_\mu\mu_-\pi_dn_s}\right)^{\alpha/d} + \frac{k_u}{k} C_\alpha\left(\frac{2k_u}{c_\mu^*\mu_-\pi_dn_u}\right)^{\alpha/d}
% \right)^{{1+\beta}}\\
% & \approx  \left(C_1\left(\frac{k_s+k_s^2}{k^2}\right)^{1/4}+C_2\left(\frac{k_u+k_u^2}{k^2}\right)^{1/2}+C_3 k_s  \left(\frac{k_s}{c_\mu n_s}\right)^{\alpha /{d}} +C_3 k_u \left(\frac{k_u}{c_\mu^* n_u}\right)^{\alpha /{d}}  \right)^{{1+\beta}}
% \end{aligned}
% \end{equation}
Finally, the excess error under the covariate shift setting can be bounded by
\begin{equation}
\begin{aligned}
\mathcal{E}_U(\hat{f})&\leq 2C_\beta\left( 
(1/k)^{1/4}
+ \frac{k_s}{k}C_\alpha\left(\frac{2k_s}{c_\mu\mu_-\pi_dn_s}\right)^{\alpha/d} + \frac{k_u}{k} C_\alpha\left(\frac{2k_u}{c_\mu^*\mu_-\pi_dn_u}\right)^{\alpha/d}
\right)^{{1+\beta}}\\
& \approx  \left(\left(\frac{1}{k}\right)^{1/4}+C_1 k_s  \left(\frac{k_s}{c_\mu n_s}\right)^{\alpha /{d}} +C_1 k_u \left(\frac{k_u}{c_\mu^* n_u}\right)^{\alpha /{d}}  \right)^{{1+\beta}}
\end{aligned}
\label{bound:28}
\end{equation}
Compared \myref{bound:28} to \myref{bound:22}, it is easy to verify that
\begin{equation}
\begin{aligned}
& \frac{k}{k}C_\alpha\left(\frac{2k}{c_\mu\mu_-\pi_dn_s}\right)^{\alpha /{d}}-\frac{k_s}{k}C_\alpha\left(\frac{2k_s}{c_\mu\mu_-\pi_dn_s}\right)^{\alpha/d} - \frac{k_u}{k} C_\alpha\left(\frac{2k_u}{c_\mu^*\mu_-\pi_dn_u}\right)^{\alpha/d}\\
&\geq \frac{k_u}{k}C_\alpha\left(\frac{2k_s}{c_\mu\mu_-\pi_dn_s}\right)^{\alpha/d}- \frac{k_u}{k} C_\alpha\left(\frac{2k_u}{c_\mu^*\mu_-\pi_dn_u}\right)^{\alpha/d}
\end{aligned}
\end{equation}
Because in general, we have $c_\mu^*\gg c_u$, the difference is then larger than $0$, namely incorporating target samples into the KNN memory bank, the excess error can be further reduced. When $\mathbbm{D}_S$ is very close to $\mathbbm{D}_U$, that is, $c_\mu^*\approx c_\mu$, the two bounds will be similar. With the assumption $k_s+k_u=k$, and $k_s=n_s^{\delta_s},k_u=n_u^{\delta_u}$, with probability at least $\min\{ 1-\exp(-(n_s^{\delta_s}+n_u^{\delta_u})/4),  1-2\exp(-2\sqrt{n_s^{\delta_s}+n_u^{\delta_u}})\}$, we have
\begin{equation}
\mathcal{E}_U(\hat{f})\leq \left(\left(\frac{1}{n_s^{\delta_s}+n_u^{\delta_u}}\right)^{1/4}+C_1 \frac{n_s^{\delta_s}}{n_s^{\delta_s}+n_u^{\delta_u}}  \left(\frac{1}{c_\mu n_s^{1-\delta_s}}\right)^{\alpha /{d}} +C_1 \frac{n_u^{\delta_u}}{n_s^{\delta_s}+n_u^{\delta_u}} \left(\frac{1}{c_\mu^* n_u^{1-\delta_u}}\right)^{\alpha /{d}}  \right)^{{1+\beta}}
\end{equation}

Similar results can be derived under the posterior-shift setting. Under the assumption that $\mathbb{E}_{Y|X}[y_u^{(i)}]=\eta_U(x_u^{(i)})$ and $\sup_{x_u\in \mathbbm{D}_U} |\eta_S(x_u)-\eta_U(x_u)|\leq C_{ada}$, we have

\begin{equation}
\begin{aligned}
\left|\hat{\eta}_k(x_u) -\eta_U(x_u) \right |&=\left| \frac{1}{k}\sum_{i=1}^{k_s} y_s^{(i)}-\frac{1}{k}\sum_{i=1}^{k_s}\eta_U(x_u) +\frac{1}{k}\sum_{i=1}^{k_u} y_u^{(i)}-\frac{1}{k}\sum_{i=1}^{k_u}\eta_U(x_u)  \right|\\
& \leq \left|\frac{1}{k}\sum_{i=1}^{k_s} y_s^{(i)}-\frac{1}{k}\sum_{i=1}^{k_s} \eta_S\left(x_s^{(i)}\right)\right|+\left| \frac{1}{k}\sum_{i=1}^{k_s} \eta_S\left(x_s^{(i)}\right)-\frac{k_s}{k}\eta_U(x_u)  \right|\\
&\quad\quad\quad +\left|\frac{1}{k}\sum_{i=1}^{k_u} y_u^{(i)}-\frac{1}{k}\sum_{i=1}^{k_u} \eta_U\left(x_u^{(i)}\right)\right|+\left| \frac{1}{k}\sum_{i=1}^{k_u} \eta_U\left(x_u^{(i)}\right)-\frac{k_u}{k}\eta_U(x_u)  \right|\\
% &\leq \underbrace{\frac{1}{k}\left|\sum_{i=1}^{k_s} y_s^{(i)}-\sum_{i=1}^{k_s}\eta\left(x_s^{(i)}\right)\right|}_{\rm \circled{\rm 1}}+\underbrace{\frac{1}{k}\sum_{i=1}^{k_s}\left| \eta\left(x_s^{(i)}\right)-\eta(x_u)  \right|}_{\rm \circled{\rm 2}}\\
% &\quad\quad\quad + \underbrace{\frac{1}{k}\left| \sum_{i=1}^{k_u}y_u^{(i)}-\sum_{i=1}^{k_u}\eta\left(x_u^{(i)}\right)\right|}_{\rm \circled{\rm 3}}+\underbrace{\frac{1}{k}\sum_{i=1}^{k_u}\left| \eta\left(x_u^{(i)}\right)-\eta(x_u)  \right|}_{\rm \circled{}}
&\leq \frac{1}{k}\left|\sum_{i=1}^{k_s} y_s^{(i)}+\sum_{i=1}^{k_u}y_u^{(i)}-\sum_{i=1}^{k_s}\eta_S\left(x_s^{(i)}\right)-\sum_{i=1}^{k_u}\eta_U\left(x_u^{(i)}\right)\right|+\frac{1}{k}\sum_{i=1}^{k_s}\left| \eta_S\left(x_s^{(i)}\right)-\eta_S(x_u)  \right|\\
&\quad\quad\quad+\frac{1}{k}\sum_{i=1}^{k_u}\left| \eta_U\left(x_u^{(i)}\right)-\eta_U(x_u)  \right| + \frac{k_s}{k}\left|\eta_S(x_u)-\eta_U(x_u)  \right|,
\end{aligned}
\end{equation}
and the conclusion will be
\begin{equation}
\begin{aligned}
\mathcal{E}_U(\hat{f})&\leq 2C_\beta\left( 
(1/k)^{1/4}
+ \frac{k_s}{k}C_\alpha\left(\frac{2k_s}{c_\mu\mu_-\pi_dn_s}\right)^{\alpha/d} + \frac{k_u}{k} C_\alpha\left(\frac{2k_u}{c_\mu^*\mu_-\pi_dn_u}\right)^{\alpha/d} +
\frac{k_s}{k} C_{ada}
\right)^{{1+\beta}}\\
&\approx \left(\left(\frac{1}{n_s^{\delta_s}+n_u^{\delta_u}}\right)^{1/4}+\frac{C_1}{n_s^{\delta_s}+n_u^{\delta_u}}\left( n_s^{\delta_s}\left(\frac{1}{c_\mu n_s^{1-\delta_s}}\right)^{\alpha /{d}} + n_u^{\delta_u} \left(\frac{1}{c_\mu^* n_u^{1-\delta_u}}\right)^{\alpha /{d}}\right) + \frac{n_s^{\delta_s}}{n_s^{\delta_s}+n_u^{\delta_u}} C_{ada} \right)^{{1+\beta}}
\end{aligned}
\end{equation}
holds with probability at least $\min\{ 1-\exp(-(n_s^{\delta_s}+n_u^{\delta_u})/4),  1-2\exp(-2\sqrt{n_s^{\delta_s}+n_u^{\delta_u}})\}$.

\subsection{Theoretical intuition for choosing the best $k$}
{\color{red} is it reasonable?}
According to \myref{bound:22}, the excess error is bounded by
\begin{equation}
\mathcal{E}_U(\hat{f})\leq \left(\left(\frac{1}{k}\right)^{1/4}+C_1  \left(\frac{k}{c_\mu n_s}\right)^{\alpha /{d}} \right)^{{1+\beta}},
\end{equation}
Our target is to find the best $k^*$ that $k^*=\arg\min_k \left(\frac{1}{k}\right)^{1/4}+C_1  \left(\frac{k}{c_\mu n_s}\right)^{\alpha /{d}}$. The first derivative and second derivative are with respect to $k$ is
\begin{equation}
\begin{aligned}
&\frac{\partial \mathcal{E}_U(\hat{f})^{-1-\beta}}{\partial k}=-\frac{1}{4}\left(\frac{1}{k}\right)^{-5/4}+\frac{C_1}{c_\mu n_s}\frac{\alpha}{d}\left(\frac{k}{c_\mu n_s}\right)^{\alpha /{d}-1}\\
&\frac{\partial^2 \mathcal{E}_U(\hat{f})^{-1-\beta}}{\partial k}=\frac{5}{16}\left(\frac{1}{k}\right)^{-9/4}+\frac{C_1}{c_\mu^2 n_s^2}\frac{\alpha}{d}(\frac{\alpha}{d}-1)\left(\frac{k}{c_\mu n_s}\right)^{\alpha /{d}-2}\\
\end{aligned}
\end{equation}
When $\frac{\partial \mathcal{E}_U(\hat{f})^{-1-\beta}}{\partial k}=0$, we have $k=\left(\left(\frac{1}{c_\mu n_s}\right)^{\alpha/d}\frac{4\alpha C_1}{d}\right)^{1/4+\alpha/d}$

\section{Dataset and implementation details}\label{sec:data_detail}
\subsection{Dataset Details}

\textbf{Rotated MNIST} \cite{ghifary2015domain} consists of 10,000 digits in MNIST with different rotated angles where the domain is determined by the degrees $d \in \{0, 15, 30, 45,
60, 75\}$.

\textbf{PACS} \cite{li2017deeper} includes 9, 991 images with 7 classes $y \in  \{$ dog, elephant, giraffe, guitar, horse, house, person $\}$ from 4 domains $d \in$ $\{$art, cartoons, photos, sketches$\}$. 

\textbf{VLCS} \cite{torralba2011unbiased} is composed of 10,729 images, 5 classes $y \in \{$ bird, car, chair, dog, person $\}$ from domains $d \in \{$Caltech101, LabelMe, SUN09, VOC2007$\}$. 

\textbf{TerraIncognita}~\cite{beery2018recognition} contains photographs of wild animals taken by camera traps at locations $d\in \{L100,L38, L43, L46\}$, with $24,788$ examples of dimension $(3,224,224)$ and $10$ classes.

\textbf{DomainNet}~\cite{peng2019moment} has six domains $d \in$ $\{$clipart, infograph, painting, quickdraw, real, sketch$\}$. This dataset contains $586,575$ examples of sizes $(3,224,224)$ and $345$ classes.

\subsection{implementation and hyper-parameter details}

\textbf{Hyperparameter search.} Following the experimental settings in \cite{gulrajani2021in}, we conduct a random search of 20 trials over the hyperparameter distribution for each algorithm and test domain. Specifically, we split the data from each domain into $80\%$ and $20\%$ proportions, where the larger split is used for training and evaluation, and the smaller ones are used for select hyperparameters. Finally, we report the mean over these repetitions as well as their estimated standard error. 

\textbf{Model selection.} The model selection in domain generalization is intrinsically a learning problem, and we use both the test-domain and Training-domain validation methods, two of the three selection methods in \cite{gulrajani2021in}. The test-domain validation strategy is an oracle-selection one since we choose the model maximizing the accuracy on a validation set that follows the distribution of the test domain.

\textbf{Model architectures.}
%\subsection{Model Architectures} \label{app:gan} \textbf{Encoders.}
Following \cite{gulrajani2021in}, we use ConvNet (Table.\ref{tab:convnet}) as the encoder for RotatedMNIST (detailed in Appendix D.1 in \cite{gulrajani2021in}) with MIT License. For other datasets, torch-vision for ResNet18 and ResNet50 (Apache-2.0), \textit{timm} for Vision Transformer (Apache-2.0), and the official repository of T3A (MIT License) are used.
\begin{table}
\centering
% \footnotesize
%\begin{table}[]
\begin{tabular}{@{}ll@{}}
\toprule
\# & Layer                                                     \\ \midrule
1  & \cellcolor[HTML]{FFFFFF}Conv2D (in=d, out=64)             \\
2  & \cellcolor[HTML]{FFFFFF}ReLU                              \\
3  & \cellcolor[HTML]{FFFFFF}GroupNorm (groups=8)              \\
4  & \cellcolor[HTML]{FFFFFF}Conv2D (in=64, out=128, stride=2) \\
5  & \cellcolor[HTML]{FFFFFF}ReLU                              \\
6  & \cellcolor[HTML]{FFFFFF}GroupNorm (8 groups)              \\
7  & \cellcolor[HTML]{FFFFFF}Conv2D (in=128, out=128)          \\
8  & \cellcolor[HTML]{FFFFFF}ReLU                              \\
9  & \cellcolor[HTML]{FFFFFF}GroupNorm (8 groups)              \\
10 & \cellcolor[HTML]{FFFFFF}Conv2D (in=128, out=128)          \\
11 & \cellcolor[HTML]{FFFFFF}ReLU                              \\
12 & \cellcolor[HTML]{FFFFFF}GroupNorm (8 groups)              \\
13 & \cellcolor[HTML]{FFFFFF}Global average-pooling            \\ \bottomrule
\end{tabular}
\caption{Details of our MNIST ConvNet architecture. All convolutions use 3×3 kernels and ``same'' padding}\label{tab:convnet}
%\end{table}
\end{table}
We run our experiments mainly on Tesla-V100 (32G)x4 instances.
\section{Additional Experimental Results}\label{sec:addexp}

\subsection{Detailed Generalization Results}

Tables~\ref{tab:rotatedmnist},~\ref{tab:vlcs},~\ref{tab:pacs},~\ref{tab:domainnet}contain detailed results for each dataset with ’Test-domain’ and ’Training-domain’ model selection methods.

\begin{table}[t]
\caption{ Domain generalization accuracy (\%) on Rotated MNIST.}
\begin{center}
\adjustbox{max width=\textwidth}{%
\begin{tabular}{lccccccc}
% \specialrule{0em}{8pt}{0pt}
\toprule
\multicolumn{8}{c}{\textbf{Rotated MNIST, Model selection: ‘Test-domain’ validation set}}\\
\textbf{Algorithm}   & \textbf{0}           & \textbf{15}          & \textbf{30}          & \textbf{45}          & \textbf{60}          & \textbf{75}          & \textbf{Avg}         \\
\midrule
ERM~\cite{vapnik1998statistical}                  & 95.3 $\pm$ 0.2       & 98.7 $\pm$ 0.1       & 98.9 $\pm$ 0.1       & 98.7 $\pm$ 0.2       & 98.9 $\pm$ 0.0       & 96.2 $\pm$ 0.2       & 97.8                 \\
IRM~\cite{arjovsky2020invariant}                  & 94.9 $\pm$ 0.6       & 98.7 $\pm$ 0.2       & 98.6 $\pm$ 0.1       & 98.6 $\pm$ 0.2       & 98.7 $\pm$ 0.1       & 95.2 $\pm$ 0.3       & 97.5                 \\
GDRO~\cite{sagawa2020distributionally}             & 95.9 $\pm$ 0.1       & 99.0 $\pm$ 0.1       & 98.9 $\pm$ 0.1       & 98.8 $\pm$ 0.1       & 98.6 $\pm$ 0.1       & 96.3 $\pm$ 0.4       & 97.9                 \\
Mixup~\cite{yan2020improve}                & 95.8 $\pm$ 0.3       & 98.7 $\pm$ 0.0       & 99.0 $\pm$ 0.1       & 98.8 $\pm$ 0.1       & 98.8 $\pm$ 0.1       & 96.6 $\pm$ 0.2       & 98.0                 \\
MLDG~\cite{li2018learning}                 & 95.7 $\pm$ 0.2       & 98.9 $\pm$ 0.1       & 98.8 $\pm$ 0.1       & 98.9 $\pm$ 0.1       & 98.6 $\pm$ 0.1       & 95.8 $\pm$ 0.4       & 97.8                 \\
CORAL~\cite{sun2016deep}                & 96.2 $\pm$ 0.2       & 98.8 $\pm$ 0.1       & 98.8 $\pm$ 0.1       & 98.8 $\pm$ 0.1       & 98.9 $\pm$ 0.1       & 96.4 $\pm$ 0.2       & 98.0                 \\
MMD~\cite{li2018domain}                  & 96.1 $\pm$ 0.2       & 98.9 $\pm$ 0.0       & 99.0 $\pm$ 0.0       & 98.8 $\pm$ 0.0       & 98.9 $\pm$ 0.0       & 96.4 $\pm$ 0.2       & 98.0                 \\
DANN~\cite{ganin2016domain}                 & 95.9 $\pm$ 0.1       & 98.9 $\pm$ 0.1       & 98.6 $\pm$ 0.2       & 98.7 $\pm$ 0.1       & 98.9 $\pm$ 0.0       & 96.3 $\pm$ 0.3       & 97.9                 \\
CDANN~\cite{li2018deep}               & 95.9 $\pm$ 0.2       & 98.8 $\pm$ 0.0       & 98.7 $\pm$ 0.1       & 98.9 $\pm$ 0.1       & 98.8 $\pm$ 0.1       & 96.1 $\pm$ 0.3       & 97.9                 \\
MTL~\cite{blanchard2021domain}                  & 96.1 $\pm$ 0.2       & 98.9 $\pm$ 0.0       & 99.0 $\pm$ 0.0       & 98.7 $\pm$ 0.1       & 99.0 $\pm$ 0.0       & 95.8 $\pm$ 0.3       & 97.9                 \\
SagNet~\cite{nam2021reducing}               & 95.9 $\pm$ 0.1       & 99.0 $\pm$ 0.1       & 98.9 $\pm$ 0.1       & 98.6 $\pm$ 0.1       & 98.8 $\pm$ 0.1       & 96.3 $\pm$ 0.1       & 97.9                 \\
ARM~\cite{zhang2021adaptive}                  & 95.9 $\pm$ 0.4       & 99.0 $\pm$ 0.1       & 98.8 $\pm$ 0.1       & 98.9 $\pm$ 0.1       & 99.1 $\pm$ 0.1       & 96.7 $\pm$ 0.2       & 98.1                 \\
VREx~\cite{krueger2021out}                 & 95.5 $\pm$ 0.2       & 99.0 $\pm$ 0.0       & 98.7 $\pm$ 0.2       & 98.8 $\pm$ 0.1       & 98.8 $\pm$ 0.0       & 96.4 $\pm$ 0.0       & 97.9                 \\
RSC~\cite{huang2020self}                  & 95.4 $\pm$ 0.1       & 98.6 $\pm$ 0.1       & 98.6 $\pm$ 0.1       & 98.9 $\pm$ 0.0       & 98.8 $\pm$ 0.1       & 95.4 $\pm$ 0.3       & 97.6                 \\
Fish~\cite{shi2022gradient}&        &       &        &        &       &        & 97.9                \\
Fisher~\cite{rame2022fishr} & 95.8 $\pm$ 0.1       & 98.3 $\pm$ 0.1       & 98.8 $\pm$ 0.1       & 98.6 $\pm$ 0.3       & 98.7 $\pm$ 0.1       & 96.5 $\pm$ 0.1       & 97.8              \\
% DRM~\cite{zhang2022domain}                   & 96.4 $\pm$ 0.2       & 98.4 $\pm$ 0.0       & 98.9 $\pm$ 0.2       & 99.0 $\pm$ 0.2       & 98.9 $\pm$ 0.2       & 96.8 $\pm$ 0.2       & 98.1                 \\
\rowcolor{Gray}
\knn                   & {97.2 $\pm$ 0.1}       & \textbf{99.2 $\pm$ 0.0}       & \textbf{99.1 $\pm$ 0.0}       & \textbf{99.0 $\pm$ 0.1}       & \textbf{99.2 $\pm$ 0.0}       & \textbf{97.6 $\pm$ 0.1}       & \textbf{98.5}                 \\
\rowcolor{Gray}
\knn+NP                   & \textbf{97.4 $\pm$ 0.1}       & {99.0 $\pm$ 0.0}       & {98.8 $\pm$ 0.0}       & {98.8 $\pm$ 0.1}       & {99.0 $\pm$ 0.1}       & {97.3 $\pm$ 0.1}       & {98.4}                 \\

\bottomrule
\multicolumn{8}{c}{\textbf{Rotated MNIST, Model selection: ‘Training-domain’ validation set}}\\
\textbf{Algorithm}   & \textbf{0}           & \textbf{15}          & \textbf{30}          & \textbf{45}          & \textbf{60}          & \textbf{75}          & \textbf{Avg}         \\
\midrule
ERM~\cite{vapnik1998statistical}                  & 95.9 $\pm$ 0.1       & 98.9 $\pm$ 0.0       & 98.8 $\pm$ 0.0       & 98.9 $\pm$ 0.0       & 98.9 $\pm$ 0.0       & 96.4 $\pm$ 0.0       & 98.0                 \\
IRM~\cite{arjovsky2020invariant}                   & 95.5 $\pm$ 0.1       & 98.8 $\pm$ 0.2       & 98.7 $\pm$ 0.1       & 98.6 $\pm$ 0.1       & 98.7 $\pm$ 0.0       & 95.9 $\pm$ 0.2       & 97.7                 \\
GDRO~\cite{sagawa2020distributionally}             & 95.6 $\pm$ 0.1       & 98.9 $\pm$ 0.1       & 98.9 $\pm$ 0.1       & 99.0 $\pm$ 0.0       & 98.9 $\pm$ 0.0       & 96.5 $\pm$ 0.2       & 98.0                 \\
Mixup~\cite{yan2020improve}                & 95.8 $\pm$ 0.3       & 98.9 $\pm$ 0.0       & 98.9 $\pm$ 0.0       & 98.9 $\pm$ 0.0       & 98.8 $\pm$ 0.1       & 96.5 $\pm$ 0.3       & 98.0                 \\
MLDG~\cite{li2018learning}                 & 95.8 $\pm$ 0.1       & 98.9 $\pm$ 0.1       & 99.0 $\pm$ 0.0       & 98.9 $\pm$ 0.1       & 99.0 $\pm$ 0.0       & 95.8 $\pm$ 0.3       & 97.9                 \\
CORAL~\cite{sun2016deep}                & 95.8 $\pm$ 0.3       & 98.8 $\pm$ 0.0       & 98.9 $\pm$ 0.0       & 99.0 $\pm$ 0.0       & 98.9 $\pm$ 0.1       & 96.4 $\pm$ 0.2       & 98.0                 \\
MMD~\cite{li2018domain}                  & 95.6 $\pm$ 0.1       & 98.9 $\pm$ 0.1       & 99.0 $\pm$ 0.0       & 99.0 $\pm$ 0.0       & 98.9 $\pm$ 0.0       & 96.0 $\pm$ 0.2       & 97.9                 \\
DANN~\cite{ganin2016domain}                 & 95.0 $\pm$ 0.5       & 98.9 $\pm$ 0.1       & 99.0 $\pm$ 0.0       & 99.0 $\pm$ 0.1       & 98.9 $\pm$ 0.0       & 96.3 $\pm$ 0.2       & 97.8                 \\
CDANN~\cite{li2018deep}                & 95.7 $\pm$ 0.2       & 98.8 $\pm$ 0.0       & 98.9 $\pm$ 0.1       & 98.9 $\pm$ 0.1       & 98.9 $\pm$ 0.1       & 96.1 $\pm$ 0.3       & 97.9                 \\
MTL~\cite{blanchard2021domain}                  & 95.6 $\pm$ 0.1       & 99.0 $\pm$ 0.1       & 99.0 $\pm$ 0.0       & 98.9 $\pm$ 0.1       & 99.0 $\pm$ 0.1       & 95.8 $\pm$ 0.2       & 97.9                 \\
SagNet~\cite{nam2021reducing}                & 95.9 $\pm$ 0.3       & 98.9 $\pm$ 0.1       & 99.0 $\pm$ 0.1       & \textbf{99.1 $\pm$ 0.0}       & 99.0 $\pm$ 0.1       & 96.3 $\pm$ 0.1       & 98.0                 \\
ARM~\cite{zhang2021adaptive}                  & 96.7 $\pm$ 0.2       & 99.1 $\pm$ 0.0       & 99.0 $\pm$ 0.0       & 99.0 $\pm$ 0.1       & {99.1 $\pm$ 0.1}       & 96.5 $\pm$ 0.4       & 98.2                 \\
VREx~\cite{krueger2021out}                 & 95.9 $\pm$ 0.2       & 99.0 $\pm$ 0.1       & 98.9 $\pm$ 0.1       & 98.9 $\pm$ 0.1       & 98.7 $\pm$ 0.1       & 96.2 $\pm$ 0.2       & 97.9                 \\
RSC~\cite{huang2020self}                  & 94.8 $\pm$ 0.5       & 98.7 $\pm$ 0.1       & 98.8 $\pm$ 0.1       & 98.8 $\pm$ 0.0       & 98.9 $\pm$ 0.1       & 95.9 $\pm$ 0.2       & 97.6                 \\
Fish~\cite{shi2022gradient}&        &       &        &        &       &        & 98.0                \\
Fisher~\cite{rame2022fishr}  & 95.0 $\pm$ 0.3       & 98.5 $\pm$ 0.0       & \textbf{99.2 $\pm$ 0.1}       & 98.9 $\pm$ 0.0       & 98.9 $\pm$ 0.1       & 96.5 $\pm$ 0.1       & 97.8                 \\
% DRM~\cite{zhang2022domain}                  &        &       &        &        &       &        & 98.0                \\
\rowcolor{Gray}
\knn                   & {97.7 $\pm$ 0.4}       & \textbf{99.1 $\pm$ 0.0}       & 99.1 $\pm$ 0.1       & \textbf{99.1 $\pm$ 0.1 }      & \textbf{99.2 $\pm$ 0.0 }      & {97.5 $\pm$ 0.2}       & {98.6 }                \\
\rowcolor{Gray}
\knn+BN                   & \textbf{97.9 $\pm$ 0.3}       & \textbf{99.1 $\pm$ 0.1}       & \textbf{99.2 $\pm$ 0.0}       & \textbf{99.1 $\pm$ 0.1}       & \textbf{99.2 $\pm$ 0.0}       & \textbf{98.0 $\pm$ 0.4}       & \textbf{98.8}                 \\
\bottomrule

\end{tabular}}
\end{center}
\label{tab:rotatedmnist}
\end{table}

\begin{table}[b]
\caption{ Domain generalization accuracy (\%) on VLCS.}
\begin{center}
\adjustbox{max width=\textwidth}{%
\setlength{\tabcolsep}{7.25pt}
\begin{tabular}{lccccc}
\toprule
\multicolumn{6}{c}{\textbf{VLCS, Model selection: ‘Test-domain’ validation set}}\\
\textbf{Algorithm}   & \textbf{C}           & \textbf{L}           & \textbf{S}           & \textbf{V}           & \textbf{Avg}         \\
\midrule
ERM~\cite{vapnik1998statistical}                  & 97.6 $\pm$ 0.3       & 67.9 $\pm$ 0.7       & 70.9 $\pm$ 0.2       & 74.0 $\pm$ 0.6       & 77.6                 \\
IRM~\cite{arjovsky2020invariant}                  & 97.3 $\pm$ 0.2       & 66.7 $\pm$ 0.1       & 71.0 $\pm$ 2.3       & 72.8 $\pm$ 0.4       & 76.9                 \\
GDRO~\cite{sagawa2020distributionally}             & 97.7 $\pm$ 0.2       & 65.9 $\pm$ 0.2       & 72.8 $\pm$ 0.8       & 73.4 $\pm$ 1.3       & 77.4                 \\
Mixup~\cite{yan2020improve}                & 97.8 $\pm$ 0.4       & 67.2 $\pm$ 0.4       & 71.5 $\pm$ 0.2       & 75.7 $\pm$ 0.6       & 78.1                 \\
MLDG~\cite{li2018learning}                 & 97.1 $\pm$ 0.5       & 66.6 $\pm$ 0.5       & 71.5 $\pm$ 0.1       & 75.0 $\pm$ 0.9       & 77.5                 \\
CORAL~\cite{sun2016deep}                & 97.3 $\pm$ 0.2       & 67.5 $\pm$ 0.6       & 71.6 $\pm$ 0.6       & 74.5 $\pm$ 0.0       & 77.7                 \\
MMD~\cite{li2018domain}                  & 98.8 $\pm$ 0.0       & 66.4 $\pm$ 0.4       & 70.8 $\pm$ 0.5       & 75.6 $\pm$ 0.4       & 77.9                 \\
DANN~\cite{ganin2016domain}                 & 99.0 $\pm$ 0.2       & 66.3 $\pm$ 1.2       & 73.4 $\pm$ 1.4       & 80.1 $\pm$ 0.5       & 79.7                 \\
CDANN~\cite{li2018deep}               & 98.2 $\pm$ 0.1       & 68.8 $\pm$ 0.5       & 74.3 $\pm$ 0.6       & 78.1 $\pm$ 0.5       & 79.9                 \\
MTL~\cite{blanchard2021domain}                  & 97.9 $\pm$ 0.7       & 66.1 $\pm$ 0.7       & 72.0 $\pm$ 0.4       & 74.9 $\pm$ 1.1       & 77.7                 \\
SagNet~\cite{nam2021reducing}               & 97.4 $\pm$ 0.3       & 66.4 $\pm$ 0.4       & 71.6 $\pm$ 0.1       & 75.0 $\pm$ 0.8       & 77.6                 \\
ARM~\cite{zhang2021adaptive}                  & 97.6 $\pm$ 0.6       & 66.5 $\pm$ 0.3       & 72.7 $\pm$ 0.6       & 74.4 $\pm$ 0.7       & 77.8                 \\
VREx~\cite{krueger2021out}                 & 98.4 $\pm$ 0.2       & 66.4 $\pm$ 0.7       & 72.8 $\pm$ 0.1       & 75.0 $\pm$ 1.4       & 78.1                 \\
RSC~\cite{huang2020self}                  & 98.0 $\pm$ 0.4       & 67.2 $\pm$ 0.3       & 70.3 $\pm$ 1.3       & 75.6 $\pm$ 0.4       & 77.8                 \\
Fish~\cite{shi2022gradient} &       &       &  &  &         77.8      \\
Fisher~\cite{rame2022fishr} & 97.6 $\pm$ 0.7       & 67.3 $\pm$ 0.5       & 72.2 $\pm$ 0.9       & 75.7 $\pm$ 0.3       & 78.2    \\
% DRM~\cite{zhang2022domain} & 97.5 $\pm$ 0.2       & 71.8 $\pm$ 1.2      & 76.6 $\pm$ 0.3       & 76.4 $\pm$ 1.0 &   80.5              \\
\rowcolor{Gray}
\knn                & \textbf{98.7 $\pm$ 0.2}       & 66.6 $\pm$ 0.2      & 74.6 $\pm$ 0.3       & 79.6 $\pm$ 0.5    &79.9            \\
\rowcolor{Gray}
+BN retraining                & \textbf{98.7 $\pm$ 0.2}       & \textbf{67.4 $\pm$ 0.3}      &\textbf{ 74.9 $\pm$ 0.5}       & \textbf{79.7 $\pm$ 0.5}    &\textbf{80.2 }           \\\midrule
\multicolumn{6}{c}{\textbf{VLCS, Model selection: ‘Training-domain’ validation set}}\\
\textbf{Algorithm}   & \textbf{C}           & \textbf{L}           & \textbf{S}           & \textbf{V}           & \textbf{Avg}         \\
\midrule
ERM~\cite{vapnik1998statistical}                 & 97.7 $\pm$ 0.4       & 64.3 $\pm$ 0.9       & 73.4 $\pm$ 0.5       & 74.6 $\pm$ 1.3       & 77.5                 \\
IRM~\cite{arjovsky2020invariant}              & 98.6 $\pm$ 0.1       & 64.9 $\pm$ 0.9       & 73.4 $\pm$ 0.6       & 77.3 $\pm$ 0.9       & 78.5                 \\
GDRO~\cite{sagawa2020distributionally}          & 97.3 $\pm$ 0.3       & 63.4 $\pm$ 0.9       & 69.5 $\pm$ 0.8       & 76.7 $\pm$ 0.7       & 76.7                 \\
Mixup~\cite{yan2020improve}            & 98.3 $\pm$ 0.6       & 64.8 $\pm$ 1.0       & 72.1 $\pm$ 0.5       & 74.3 $\pm$ 0.8       & 77.4                 \\
MLDG~\cite{li2018learning}             & 97.4 $\pm$ 0.2       & 65.2 $\pm$ 0.7       & 71.0 $\pm$ 1.4       & 75.3 $\pm$ 1.0       & 77.2                 \\
CORAL~\cite{sun2016deep}            & 98.3 $\pm$ 0.1       & 66.1 $\pm$ 1.2       & 73.4 $\pm$ 0.3       & 77.5 $\pm$ 1.2       & 78.8                 \\
MMD~\cite{li2018domain}              & 97.7 $\pm$ 0.1       & 64.0 $\pm$ 1.1       & 72.8 $\pm$ 0.2       & 75.3 $\pm$ 3.3       & 77.5                 \\
DANN~\cite{ganin2016domain}              & \textbf{99.0 $\pm$ 0.3}       & 65.1 $\pm$ 1.4       & 73.1 $\pm$ 0.3       & 77.2 $\pm$ 0.6       & 78.6                 \\
CDANN~\cite{li2018deep}         & 97.1 $\pm$ 0.3       & 65.1 $\pm$ 1.2       & 70.7 $\pm$ 0.8       & 77.1 $\pm$ 1.5       & 77.5                 \\
MTL~\cite{blanchard2021domain}              & 97.8 $\pm$ 0.4       & 64.3 $\pm$ 0.3       & 71.5 $\pm$ 0.7       & 75.3 $\pm$ 1.7       & 77.2                 \\
SagNet~\cite{nam2021reducing}           & 97.9 $\pm$ 0.4       & 64.5 $\pm$ 0.5       & 71.4 $\pm$ 1.3       & 77.5 $\pm$ 0.5       & 77.8                 \\
ARM~\cite{zhang2021adaptive}              & 98.7 $\pm$ 0.2       & 63.6 $\pm$ 0.7       & 71.3 $\pm$ 1.2       & 76.7 $\pm$ 0.6       & 77.6                 \\
VREx~\cite{krueger2021out}             & 98.4 $\pm$ 0.3       & 64.4 $\pm$ 1.4       & 74.1 $\pm$ 0.4       & 76.2 $\pm$ 1.3       & 78.3                 \\
RSC~\cite{huang2020self}               & 97.9 $\pm$ 0.1       & 62.5 $\pm$ 0.7       & 72.3 $\pm$ 1.2       & 75.6 $\pm$ 0.8       & 77.1                 \\     
Fish~\cite{shi2022gradient} &       &       &  &  &         77.8      \\
Fisher~\cite{rame2022fishr} & 98.9 $\pm$ 0.3       & 64.0 $\pm$ 0.5       & 71.5 $\pm$ 0.2       & 76.8 $\pm$ 0.7       & 77.8    \\
% DRM~\cite{zhang2022domain} &       &       &  &  &         78.9      \\
\rowcolor{Gray}
\knn                & 98.9 $\pm$ 0.3       & 64.5 $\pm$ 1.0      & 73.5 $\pm$ 0.7       & 75.6 $\pm$ 0.8    &78.1            \\
\rowcolor{Gray}
+BN retraining                & 98.4 $\pm$ 0.6       & \textbf{65.2 $\pm$ 1.2}      &\textbf{ 74.4 $\pm$ 0.3}       & \textbf{77.4 $\pm$ 1.1}    &\textbf{78.9 }           \\
\bottomrule
\end{tabular}}
\end{center}
\label{tab:vlcs}
\end{table}

\begin{table}[b]
\caption{ Domain generalization accuracy (\%) on PACS.}
\begin{center}
\adjustbox{max width=\textwidth}{%
\setlength{\tabcolsep}{7.25pt}
\begin{tabular}{lccccc}
\toprule
\multicolumn{6}{c}{\textbf{PACS, Model selection: ‘Test-domain’ validation set}}\\
\textbf{Algorithm}   & \textbf{A}           & \textbf{C}           & \textbf{P}           & \textbf{S}           & \textbf{Avg}         \\
\midrule
ERM~\cite{vapnik1998statistical}                 & 86.5 $\pm$ 1.0       & 81.3 $\pm$ 0.6       & 96.2 $\pm$ 0.3       & 82.7 $\pm$ 1.1       & 86.7                 \\
IRM~\cite{arjovsky2020invariant}              & 84.2 $\pm$ 0.9       & 79.7 $\pm$ 1.5       & 95.9 $\pm$ 0.4       & 78.3 $\pm$ 2.1       & 84.5                 \\
GDRO~\cite{sagawa2020distributionally}          & 87.5 $\pm$ 0.5       & 82.9 $\pm$ 0.6       & 97.1 $\pm$ 0.3       & 81.1 $\pm$ 1.2       & 87.1                 \\
Mixup~\cite{yan2020improve}            & 87.5 $\pm$ 0.4       & 81.6 $\pm$ 0.7       & 97.4 $\pm$ 0.2       & 80.8 $\pm$ 0.9       & 86.8                 \\
MLDG~\cite{li2018learning}             & 87.0 $\pm$ 1.2       & 82.5 $\pm$ 0.9       & 96.7 $\pm$ 0.3       & 81.2 $\pm$ 0.6       & 86.8                 \\
CORAL~\cite{sun2016deep}            & 86.6 $\pm$ 0.8       & 81.8 $\pm$ 0.9       & 97.1 $\pm$ 0.5       & 82.7 $\pm$ 0.6       & 87.1                 \\
MMD~\cite{li2018domain}              & 88.1 $\pm$ 0.8       & 82.6 $\pm$ 0.7       & 97.1 $\pm$ 0.5       & 81.2 $\pm$ 1.2       & 87.2                 \\
DANN~\cite{ganin2016domain}              & 87.0 $\pm$ 0.4       & 80.3 $\pm$ 0.6       & 96.8 $\pm$ 0.3       & 76.9 $\pm$ 1.1       & 85.2                 \\
CDANN~\cite{li2018deep}         & 87.7 $\pm$ 0.6       & 80.7 $\pm$ 1.2       & 97.3 $\pm$ 0.4       & 77.6 $\pm$ 1.5       & 85.8                 \\
MTL~\cite{blanchard2021domain}              & 87.0 $\pm$ 0.2       & 82.7 $\pm$ 0.8       & 96.5 $\pm$ 0.7       & 80.5 $\pm$ 0.8       & 86.7                 \\
SagNet~\cite{nam2021reducing}           & 87.4 $\pm$ 0.5       & 81.2 $\pm$ 1.2       & 96.3 $\pm$ 0.8       & 80.7 $\pm$ 1.1       & 86.4                 \\
ARM~\cite{zhang2021adaptive}              & 85.0 $\pm$ 1.2       & 81.4 $\pm$ 0.2       & 95.9 $\pm$ 0.3       & 80.9 $\pm$ 0.5       & 85.8                 \\
VREx~\cite{krueger2021out}             & 87.8 $\pm$ 1.2       & 81.8 $\pm$ 0.7       & 97.4 $\pm$ 0.2       & 82.1 $\pm$ 0.7       & 87.2                 \\
RSC~\cite{huang2020self}               & 86.0 $\pm$ 0.7       & 81.8 $\pm$ 0.9       & 96.8 $\pm$ 0.7       & 80.4 $\pm$ 0.5       & 86.2                 \\
Fish~\cite{shi2022gradient} &       &       &  &  &         85.8      \\
Fisher~\cite{rame2022fishr} & 87.9 $\pm$ 0.6       & 80.8 $\pm$ 0.5       & 97.9 $\pm$ 0.4       & 81.1 $\pm$ 0.8       & 86.9    \\
% DRM~\cite{zhang2022domain} & 87.4 $\pm$ 2.9       & 83.5 $\pm$ 0.8       & 96.0 $\pm$ 0.5       & 83.0 $\pm$ 0.7       & 87.5                 \\
\rowcolor{Gray}
\knn                & 89.1 $\pm$ 0.3       & \textbf{84.3 $\pm$ 0.1}      & \textbf{98.1 $\pm$ 0.4}       & 83.7 $\pm$ 0.5    &\textbf{88.8}           \\
\rowcolor{Gray}
\knn+NP                & \textbf{89.2 $\pm$ 0.3}       & \textbf{84.3 $\pm$ 0.1}      & 98.0 $\pm$ 0.4       & \textbf{83.8 $\pm$ 0.4}    &\textbf{88.9}           \\
\midrule
\multicolumn{6}{c}{\textbf{PACS, Model selection: ‘Training-domain’ validation set}}\\
\textbf{Algorithm}   & \textbf{A}           & \textbf{C}           & \textbf{P}           & \textbf{S}           & \textbf{Avg}         \\
\midrule
ERM~\cite{vapnik1998statistical}                 & 84.7 $\pm$ 0.4       & 80.8 $\pm$ 0.6       & 97.2 $\pm$ 0.3       & 79.3 $\pm$ 1.0       & 85.5                 \\
IRM~\cite{arjovsky2020invariant}              & 84.8 $\pm$ 1.3       & 76.4 $\pm$ 1.1       & 96.7 $\pm$ 0.6       & 76.1 $\pm$ 1.0       & 83.5                 \\
GDRO~\cite{sagawa2020distributionally}          & 83.5 $\pm$ 0.9       & 79.1 $\pm$ 0.6       & 96.7 $\pm$ 0.3       & 78.3 $\pm$ 2.0       & 84.4                 \\
Mixup~\cite{yan2020improve}            & 86.1 $\pm$ 0.5       & 78.9 $\pm$ 0.8       & 97.6 $\pm$ 0.1       & 75.8 $\pm$ 1.8       & 84.6                 \\
MLDG~\cite{li2018learning}             & 85.5 $\pm$ 1.4       & 80.1 $\pm$ 1.7       & 97.4 $\pm$ 0.3       & 76.6 $\pm$ 1.1       & 84.9                 \\
CORAL~\cite{sun2016deep}            & 88.3 $\pm$ 0.2       & 80.0 $\pm$ 0.5       & 97.5 $\pm$ 0.3       & 78.8 $\pm$ 1.3       & 86.2                 \\
MMD~\cite{li2018domain}              & 86.1 $\pm$ 1.4       & 79.4 $\pm$ 0.9       & 96.6 $\pm$ 0.2       & 76.5 $\pm$ 0.5       & 84.6                 \\
DANN~\cite{ganin2016domain}              & 86.4 $\pm$ 0.8       & 77.4 $\pm$ 0.8       & 97.3 $\pm$ 0.4       & 73.5 $\pm$ 2.3       & 83.6                 \\
CDANN~\cite{li2018deep}         & 84.6 $\pm$ 1.8       & 75.5 $\pm$ 0.9       & 96.8 $\pm$ 0.3       & 73.5 $\pm$ 0.6       & 82.6                 \\
MTL~\cite{blanchard2021domain}              & 87.5 $\pm$ 0.8       & 77.1 $\pm$ 0.5       & 96.4 $\pm$ 0.8       & 77.3 $\pm$ 1.8       & 84.6                 \\
SagNet~\cite{nam2021reducing}           & 87.4 $\pm$ 1.0       & 80.7 $\pm$ 0.6       & 97.1 $\pm$ 0.1       & 80.0 $\pm$ 0.4       & 86.3                 \\
ARM~\cite{zhang2021adaptive}              & 86.8 $\pm$ 0.6       & 76.8 $\pm$ 0.5       & 97.4 $\pm$ 0.3       & 79.3 $\pm$ 1.2       & 85.1                 \\
VREx~\cite{krueger2021out}             & 86.0 $\pm$ 1.6       & 79.1 $\pm$ 0.6       & 96.9 $\pm$ 0.5       & 77.7 $\pm$ 1.7       & 84.9                 \\
RSC~\cite{huang2020self}               & 85.4 $\pm$ 0.8       & 79.7 $\pm$ 1.8       & 97.6 $\pm$ 0.3       & 78.2 $\pm$ 1.2       & 85.2                 \\
Fish~\cite{shi2022gradient} &       &       &  &  &          85.5      \\
Fisher~\cite{rame2022fishr} & \textbf{88.4 $\pm$ 0.2}       & 78.7 $\pm$ 0.7       & 97.0 $\pm$ 0.1       & 77.8 $\pm$ 2.0       & 85.5   \\
% DRM~\cite{zhang2022domain} &       &       &  &  &        86.2    \\
\rowcolor{Gray}
\knn                & 87.1 $\pm$ 1.3       &\textbf{ 82.2 $\pm$ 0.6}      & 97.5 $\pm$ 0.4       & \textbf{81.5 $\pm$ 0.8}    &\textbf{87.1}            \\
\rowcolor{Gray}
\knn+NP                & 86.2 $\pm$ 1.2       & \textbf{82.2 $\pm$ 0.6 }     & \textbf{98.1 $\pm$ 0.1}       & 80.2 $\pm$ 1.0    &{86.7}            \\
\bottomrule
\end{tabular}}
\end{center}
\label{tab:pacs}
\end{table}

\begin{table}[t]
\caption{ Domain generalization accuracy (\%) on DomainNet.}
\begin{center}
\adjustbox{max width=\textwidth}{%
\setlength{\tabcolsep}{7.25pt}
\begin{tabular}{lccccccc}
\specialrule{0em}{8pt}{0pt}
\toprule
\multicolumn{8}{c}{\textbf{DomainNet, Model selection: ‘Test-domain’ validation set}}\\
\textbf{Algorithm}   & \textbf{clip}        & \textbf{info}        & \textbf{paint}       & \textbf{quick}       & \textbf{real}        & \textbf{sketch}      & \textbf{Avg}         \\
\midrule
ERM~\cite{vapnik1998statistical}                 & 58.1 $\pm$ 0.3       & 18.8 $\pm$ 0.3       & 46.7 $\pm$ 0.3       & 12.2 $\pm$ 0.4       & 59.6 $\pm$ 0.1       & 49.8 $\pm$ 0.4       & 40.9                 \\
IRM~\cite{arjovsky2020invariant}              & 48.5 $\pm$ 2.8       & 15.0 $\pm$ 1.5       & 38.3 $\pm$ 4.3       & 10.9 $\pm$ 0.5       & 48.2 $\pm$ 5.2       & 42.3 $\pm$ 3.1       & 33.9                 \\
GDRO~\cite{sagawa2020distributionally}          & 47.2 $\pm$ 0.5       & 17.5 $\pm$ 0.4       & 33.8 $\pm$ 0.5       & 9.3 $\pm$ 0.3        & 51.6 $\pm$ 0.4       & 40.1 $\pm$ 0.6       & 33.3                 \\
Mixup~\cite{yan2020improve}            & 55.7 $\pm$ 0.3       & 18.5 $\pm$ 0.5       & 44.3 $\pm$ 0.5       & 12.5 $\pm$ 0.4       & 55.8 $\pm$ 0.3       & 48.2 $\pm$ 0.5       & 39.2                 \\
MLDG~\cite{li2018learning}             & 59.1 $\pm$ 0.2       & 19.1 $\pm$ 0.3       & 45.8 $\pm$ 0.7       & 13.4 $\pm$ 0.3       & 59.6 $\pm$ 0.2       & 50.2 $\pm$ 0.4       & 41.2                 \\
CORAL~\cite{sun2016deep}            & 59.2 $\pm$ 0.1       & 19.7 $\pm$ 0.2       & 46.6 $\pm$ 0.3       & 13.4 $\pm$ 0.4       & 59.8 $\pm$ 0.2       & 50.1 $\pm$ 0.6       & 41.5                 \\
MMD~\cite{li2018domain}              & 32.1 $\pm$ 13.3      & 11.0 $\pm$ 4.6       & 26.8 $\pm$ 11.3      & 8.7 $\pm$ 2.1        & 32.7 $\pm$ 13.8      & 28.9 $\pm$ 11.9      & 23.4                 \\
DANN~\cite{ganin2016domain}              & 53.1 $\pm$ 0.2       & 18.3 $\pm$ 0.1       & 44.2 $\pm$ 0.7       & 11.8 $\pm$ 0.1       & 55.5 $\pm$ 0.4       & 46.8 $\pm$ 0.6       & 38.3                 \\
CDANN~\cite{li2018deep}         & 54.6 $\pm$ 0.4       & 17.3 $\pm$ 0.1       & 43.7 $\pm$ 0.9       & 12.1 $\pm$ 0.7       & 56.2 $\pm$ 0.4       & 45.9 $\pm$ 0.5       & 38.3                 \\
MTL~\cite{blanchard2021domain}              & 57.9 $\pm$ 0.5       & 18.5 $\pm$ 0.4       & 46.0 $\pm$ 0.1       & 12.5 $\pm$ 0.1       & 59.5 $\pm$ 0.3       & 49.2 $\pm$ 0.1       & 40.6                 \\
SagNet~\cite{nam2021reducing}           & 57.7 $\pm$ 0.3       & 19.0 $\pm$ 0.2       & 45.3 $\pm$ 0.3       & 12.7 $\pm$ 0.5       & 58.1 $\pm$ 0.5       & 48.8 $\pm$ 0.2       & 40.3                 \\
ARM~\cite{zhang2021adaptive}              & 49.7 $\pm$ 0.3       & 16.3 $\pm$ 0.5       & 40.9 $\pm$ 1.1       & 9.4 $\pm$ 0.1        & 53.4 $\pm$ 0.4       & 43.5 $\pm$ 0.4       & 35.5                 \\
VREx~\cite{krueger2021out}             & 47.3 $\pm$ 3.5       & 16.0 $\pm$ 1.5       & 35.8 $\pm$ 4.6       & 10.9 $\pm$ 0.3       & 49.6 $\pm$ 4.9       & 42.0 $\pm$ 3.0       & 33.6                 \\
RSC~\cite{huang2020self}               & 55.0 $\pm$ 1.2       & 18.3 $\pm$ 0.5       & 44.4 $\pm$ 0.6       & 12.2 $\pm$ 0.2       & 55.7 $\pm$ 0.7       & 47.8 $\pm$ 0.9       & 38.9  \\
Fish~\cite{shi2022gradient}                  &        &        &        &       &       &       & 43.4      \\
Fisher~\cite{rame2022fishr} & 58.3 $\pm$ 0.5       & 20.2 $\pm$ 0.2      & 47.9 $\pm$ 0.2       & 13.6 $\pm$ 0.3       & 60.5 $\pm$ 0.3       & 50.5 $\pm$ 0.3       & 41.8                 \\
% DRM~\cite{zhang2022domain}                  & 59.2 $\pm$ 0.2       & 20.8 $\pm$ 0.3      & 47.2 $\pm$ 0.1       & 15.2 $\pm$ 0.2       & 60.9 $\pm$ 0.6       & 50.8 $\pm$ 0.5       & 42.4                 \\
\rowcolor{Gray}
\knn (todo)             & 59.3 $\pm$ 0.1       & 22.0 $\pm$ 0.9       & 48.0 $\pm$ 0.9       & 15.1 $\pm$ 0.2       & 61.0 $\pm$ 0.0       & 50.9 $\pm$ 0.1       &     42.7            \\
\bottomrule
\multicolumn{8}{c}{\textbf{DomainNet, Model selection: ‘Training-domain’ validation set}}\\
\textbf{Algorithm}   & \textbf{clip}        & \textbf{info}        & \textbf{paint}       & \textbf{quick}       & \textbf{real}        & \textbf{sketch}      & \textbf{Avg}         \\
\midrule
ERM~\cite{vapnik1998statistical}                  & 58.1 $\pm$ 0.3       & 18.8 $\pm$ 0.3       & 46.7 $\pm$ 0.3       & 12.2 $\pm$ 0.4       & 59.6 $\pm$ 0.1       & 49.8 $\pm$ 0.4       & 40.9                 \\
IRM~\cite{arjovsky2020invariant}                  & 48.5 $\pm$ 2.8       & 15.0 $\pm$ 1.5       & 38.3 $\pm$ 4.3       & 10.9 $\pm$ 0.5       & 48.2 $\pm$ 5.2       & 42.3 $\pm$ 3.1       & 33.9                 \\
GDRO~\cite{sagawa2020distributionally}             & 47.2 $\pm$ 0.5       & 17.5 $\pm$ 0.4       & 33.8 $\pm$ 0.5       & 9.3 $\pm$ 0.3        & 51.6 $\pm$ 0.4       & 40.1 $\pm$ 0.6       & 33.3                 \\
Mixup~\cite{yan2020improve}                & 55.7 $\pm$ 0.3       & 18.5 $\pm$ 0.5       & 44.3 $\pm$ 0.5       & 12.5 $\pm$ 0.4       & 55.8 $\pm$ 0.3       & 48.2 $\pm$ 0.5       & 39.2                 \\
MLDG~\cite{li2018learning}                 & 59.1 $\pm$ 0.2       & 19.1 $\pm$ 0.3       & 45.8 $\pm$ 0.7       & 13.4 $\pm$ 0.3       & 59.6 $\pm$ 0.2       & 50.2 $\pm$ 0.4       & 41.2                 \\
CORAL~\cite{sun2016deep}                & 59.2 $\pm$ 0.1       & 19.7 $\pm$ 0.2       & 46.6 $\pm$ 0.3       & 13.4 $\pm$ 0.4       & 59.8 $\pm$ 0.2       & 50.1 $\pm$ 0.6       & 41.5                 \\
MMD~\cite{li2018domain}                  & 32.1 $\pm$ 13.3      & 11.0 $\pm$ 4.6       & 26.8 $\pm$ 11.3      & 8.7 $\pm$ 2.1        & 32.7 $\pm$ 13.8      & 28.9 $\pm$ 11.9      & 23.4                 \\
DANN~\cite{ganin2016domain}                 & 53.1 $\pm$ 0.2       & 18.3 $\pm$ 0.1       & 44.2 $\pm$ 0.7       & 11.8 $\pm$ 0.1       & 55.5 $\pm$ 0.4       & 46.8 $\pm$ 0.6       & 38.3                 \\
CDANN~\cite{li2018deep}                & 54.6 $\pm$ 0.4       & 17.3 $\pm$ 0.1       & 43.7 $\pm$ 0.9       & 12.1 $\pm$ 0.7       & 56.2 $\pm$ 0.4       & 45.9 $\pm$ 0.5       & 38.3                 \\
MTL~\cite{blanchard2021domain}                  & 57.9 $\pm$ 0.5       & 18.5 $\pm$ 0.4       & 46.0 $\pm$ 0.1       & 12.5 $\pm$ 0.1       & 59.5 $\pm$ 0.3       & 49.2 $\pm$ 0.1       & 40.6                 \\
SagNet~\cite{nam2021reducing}               & 57.7 $\pm$ 0.3       & 19.0 $\pm$ 0.2       & 45.3 $\pm$ 0.3       & 12.7 $\pm$ 0.5       & 58.1 $\pm$ 0.5       & 48.8 $\pm$ 0.2       & 40.3                 \\
ARM~\cite{zhang2021adaptive}                  & 49.7 $\pm$ 0.3       & 16.3 $\pm$ 0.5       & 40.9 $\pm$ 1.1       & 9.4 $\pm$ 0.1        & 53.4 $\pm$ 0.4       & 43.5 $\pm$ 0.4       & 35.5                 \\
VREx~\cite{krueger2021out}                 & 47.3 $\pm$ 3.5       & 16.0 $\pm$ 1.5       & 35.8 $\pm$ 4.6       & 10.9 $\pm$ 0.3       & 49.6 $\pm$ 4.9       & 42.0 $\pm$ 3.0       & 33.6                 \\
RSC~\cite{huang2020self}                  & 55.0 $\pm$ 1.2       & 18.3 $\pm$ 0.5       & 44.4 $\pm$ 0.6       & 12.2 $\pm$ 0.2       & 55.7 $\pm$ 0.7       & 47.8 $\pm$ 0.9       & 38.9      \\
Fish~\cite{shi2022gradient}                  &        &        &        &       &       &       & 42.7      \\
Fisher~\cite{rame2022fishr} & 58.2 $\pm$ 0.5       & 20.2 $\pm$ 0.2      & 47.7 $\pm$ 0.3       & 12.7 $\pm$ 0.2       & 60.3 $\pm$ 0.2       & 50.8 $\pm$ 0.1       & 41.7                 \\
% DRM~\cite{zhang2022domain}                  &        &        &        &       &       &       & 42.7      \\ 
\rowcolor{Gray}
\knn (todo)             & 59.3 $\pm$ 0.1       & 22.0 $\pm$ 0.9       & 48.0 $\pm$ 0.9       & 15.1 $\pm$ 0.2       & 61.0 $\pm$ 0.0       & 50.9 $\pm$ 0.1       &     42.7            \\\bottomrule
\end{tabular}}
\end{center}
\label{tab:domainnet}
\end{table}

\subsection{Extended experiments on Cifar-10-C}

~\figurename~\ref{fig:cifar10-1} shows the results with the lowest severity (one), where \knn performs the best and retraining the BN statistic will not be beneficial. For WRN-28-10 Wide ResNet Backbone, the results are shown in ~\figurename~\ref{fig:cifar10-3} and ~\figurename~\ref{fig:cifar10-4}, where the same pattern as results with 40-2 Wide ResNet Backbone are observed.

\begin{figure*}
    \centering
    \includegraphics[width=\textwidth]{imgs/severity1.pdf}
    \caption{\textbf{Corruption benchmark on CIFAR-10-C with the lowest severity (one)}. \knn+BN means that the KNN classifier and BN retraining are both used.}
    \label{fig:cifar10-1}
\end{figure*}
\begin{figure*}
    \centering
    \includegraphics[width=\textwidth]{imgs/wrn28_severity5.pdf}
    \caption{\textbf{Corruption benchmark on CIFAR-10-C with the highest severity (five) and a 40-2 Wide ResNet backbone~\cite{zagoruyko2016wide} pre-trained on CIFAR-10.} \knn+BN means that the KNN classifier and BN retraining are both used.}
    \label{fig:cifar10-3}
\end{figure*}
\begin{figure*}
    \centering
    \includegraphics[width=\textwidth]{imgs/wrn28_severity1.pdf}
    \caption{\textbf{Corruption benchmark on CIFAR-10-C with the lowest severity (one) and a 40-2 Wide ResNet backbone~\cite{zagoruyko2016wide} pre-trained on CIFAR-10}. \knn+BN means that the KNN classifier and BN retraining are both used.}
    \label{fig:cifar10-4}
\end{figure*}

\subsection{Extended Visualization of classification results.}
\figurename~\ref{fig:succ_app} provide more evaluation instances that be prediction correctly and \figurename~\ref{fig:fail_app} supplies more failure cases.
\begin{figure}
    \centering
   \includegraphics[width=\textwidth]{imgs/class_succss.pdf}
    \caption{Visualization of successfully classified results attained by \knn.}
    \label{fig:succ_app}
\end{figure}

\begin{figure}
    \centering
    \includegraphics[width=\textwidth]{imgs/class_fail.pdf}
    \caption{Visualization of misclassified results attained by \knn.}
    \label{fig:fail_app}
\end{figure}
