# Supplementary material for: Model-free Test Time Adaptation for Out-Of-Distribution Detection
Source: arXiv:2311.16420 source file (2023-11-28)
Supplement: Supplementary file 3 [file appendix_cvpr.tex]

% \section{Extended Related work}\label{sec:app_related}

% \textbf{Distribution shift.} A fundamental challenge for machine learning models is the sensitivity to changes in the data distribution. There are multiple kinds of distribution shifts such as covariate shift~\cite{gatys2016image,quinonero2008dataset,zhang2022towards, wang2022toward} (OOD samples are drawn from different input distributions); conditional label shift~\cite{arjovsky2019invariant,zhang2022domain} (the correlation between OOD samples and the corresponding labels is different from the ID distribution), or label shift (OOD samples are drawn from different classes)~\cite{hendrycks2016baseline}. All of these distribution shifts can reduce model performance~\cite{sugiyama2005input}, invalidate uncertainty estimates~\cite{ovadia2019can}, and affect model selection~\cite{sugiyama2007covariate}. Most OOD detection methods focus on the latter. 







% \begin{algorithm}[h]
%    \caption{AdaODD for the synthetic dataset in \figurename~\ref{fig:motivation2}}
%    \label{alg:main2}
%    \STATE {\bfseries Input:} ID dataset ${D}^{in}$, accessible OOD dataset ${D}^{out}=\{x_i\}_{i=1}^m$, test sample $x_{o}$, threshold $\lambda$, $k=100$ for KNN selection, sample scale $\kappa=100.$.
%    \STATE {\bfseries Initialize} the memory bank with scales $\mathcal{M}=\{x_i, s_i:=1\}_{x_i\in {D}^{in}}\bigcup \{x_i, s_i:=\kappa\}_{x_i\in {D}^{out}}$.
%    \STATE {\bfseries Inference stage for $x_{o}$.}
%     \STATE Nearest neighbors $B=\left((x_{(1)},s_{(1)}),...,(x_{k)},s_{(k)})\right)$. \\
%     \STATE Calculate score $S(x_o)=\frac{1}{k}\sum_{i=1}^k -\parallel x_o-x_{(i)} \parallel*s_{(i)}$.
%     \STATE Make desion by $\mathbf{1}\{S(x_o)\geq \lambda\}$
% \end{algorithmic}
% \end{algorithm}
% \begin{algorithm}[h]
%    \caption{AdaODD for the synthetic dataset in \figurename~\ref{fig:motivation2}}
%    \label{alg:main2}
% {\bfseries Input:} ID dataset ${D}^{in}$, accessible OOD dataset ${D}^{out}=\{x_i\}_{i=1}^m$, test sample $x_{o}$, threshold $\lambda$, $k=100$ for KNN selection, sample scale $\kappa=100.$.\\
% {\bfseries Initialize} the memory bank with scales $\mathcal{M}=\{x_i, s_i:=1\}_{x_i\in {D}^{in}}\bigcup \{x_i, s_i:=\kappa\}_{x_i\in {D}^{out}}$.\\
% {\bfseries Inference stage for $x_{o}$.}\\
%  Nearest neighbors $B=\left((x_{(1)},s_{(1)}),...,(x_{k)},s_{(k)})\right)$. \\
%  Calculate score $S(x_o)=\frac{1}{k}\sum_{i=1}^k -\parallel x_o-x_{(i)} \parallel*s_{(i)}$.\\
% Make desion by $\mathbf{1}\{S(x_o)\geq \lambda\}$\\
% \end{algorithm}

% \section{A detailed description of \figurename~\ref{fig:motivation2_acc}}\label{sec:app_teaser}

% The horizontal axis in \figurename~\ref{fig:motivation2_acc} represents the threshold value used to make the detection decision. i.e., the threshold used to classify samples as either in-distribution (ID) or out-of-distribution (OOD). In the toy example, when we choose x=1.96 as the decision boundary (classifying samples with x<1.96 as ID and x>1.96 as OOD), the detector achieves around $95\%$ accuracy on ID samples and approximately $50\%$ accuracy on OOD samples. As the decision boundary moves, the classification accuracies on both ID and OOD samples change accordingly. Specifically, when the threshold is set too high, some OOD samples may be classified as ID (false negatives), leading to an increase in ID accuracy, but a drop in OOD accuracy. Conversely, when the threshold is set too low, more OOD samples may be classified as OOD (true positives), leading to an increase in OOD accuracy, but a drop in ID accuracy as fewer ID samples are misclassified.

% The purpose of \figurename~\ref{fig:motivation2_acc} is to demonstrate that if we have some initial estimations of the OOD data, we can adjust the learned decision boundary accordingly to achieve a better trade-off in the classification of ID and OOD samples. By utilizing the test-time adaptation approach, we can leverage online test data to improve the OOD detector's performance and adjust the decision boundary dynamically based on the changing data distribution during deployment. This adaptability allows the detector to better distinguish between ID and OOD samples and achieve improved overall performance. We acknowledge that the example with two Gaussians is relatively simple and may not fully capture the complexities of real-world scenarios. Nevertheless, it serves as a conceptual demonstration of the advantages of utilizing online test instances to improve OOD detection. For real-world utility, the experimental section provides superior detection results on many large-scale benchmarks.


% \section{Theoretical justification}\label{sec:app_theory}
% % The benefits of the proposed algorithm and how we derive it is theoretically detailed in this subsection.
% \vspace{-0.15cm}
% \subsection{Log conditional
% densities score function.}\label{sec:log}
% \vspace{-0.15cm}
% To study how OOD samples influence the detection process, we partition the score function into two components, one dependent only on ID neighbors and the other dependent on selected test neighbors. Hereinafter, we treat the selected samples as low-confidence (LC) ID samples and the samples from naive ID distribution are high-confidence (HC) ID samples.  Because we do not have true labels of test samples, the LC ID sample set will contain both ID and OOD samples.\footnote{out-of-distribution samples are those which, when compared to the in-distribution, exhibit low confidence in their classification as part of the in-distribution.}. We show that, unlike previous methods that use HC ID neighbors and a fixed boundary, \abbr adjusts the boundary by the score from the LC sample information and prefers a lower false positive rate. Without access to OOD distribution, the typical decision rule is 
% \vspace{-0.1cm}
% \begin{align}
% \mathbf{I}\{S(x|{D}^{HC})\geq \lambda\},\label{eq:xue:0}
% \end{align}
% where ${D}^{HC}$ is the original ID sample set. We treat samples with scores higher than $\lambda$ as ID. The potential drawback is that the value of $\lambda$ is typically relatively small so that the in-distribution detection maintains enough accuracy. If we can access the estimated LC ID information, we may use a combined decision rule as follows:
% \begin{align}
% \mathbf{I}\{S(x|{D}^{HC}, \hat{{D}}^{LC})\ge \lambda\},\label{eq:xue:1}
% \end{align}
% where $\hat{{D}}^{LC}$ is the low-confidence ID sample set during test. Intuitively, people usually hope the score function shows similar behavior as the probability function of ID, i.e., the higher score means a higher chance/probability that the test sample $x$ is from ID. Therefore, one of the ideal choices is to set the score function being proportional to log probability, i.e., $$S(x|{D}^{HC},\hat{{D}}^{LC}) \propto \log \mathbbm{P}(x\textrm{ from ID}|{D}^{HC},\hat{{D}}^{LC}).$$
% We obtain the following equation through the maximum likelihood estimator analysis, 
% \begin{align}
% \small
% S(x|{D}^{HC},\hat{{D}}^{LC})\propto \underbrace{\sum_{x_i\in{D}^{HC}}\log p^{hc}(x|x_i)}_{(a)} + \underbrace{\sum_{x_j\in\hat{{D}}^{LC}}\log p^{lc}(x|x_j)}_{(b)},\label{eq:xue:3}
% \vspace{-0.1cm}
% \end{align}
% where $p^{hc}(\cdot)$ and $p^{lc}(\cdot)$ are the conditional density/mass function of ID given a reference sample from HC sample set and LC sample set collected during test, respectively. 
% % Note that $p^{out}$ \textbf{is not} the probability of a sample belonging to out-of-distribution, it is the conditional probability that a sample \textit{belonging to in-distribution} given a reference sample from the estimated OOD.

%  % In a typical OOD detection setting, the in-distirbution sample $N$ is much larger than the test sample size $n$. When conducting the KNN selection for the density overlapping regime, we may have a very high chance to select more in-distirbution samples. If we directly compute the log probabilities in \eqref{eq:xue:3} with all $\lambda_{in} =\lambda_{out}$, we will highly overestimate the ID density. Thus it is necessary to introduce extra coefficients to balance influence of sampling when compute the log probabilities in \eqref{eq:xue:3}.


% % The formulation \eqref{eq:xue:3} uses the sum of logarithmic conditional densities to detect ID samples. Compared to the detection rule \eqref{eq:xue:0}, the detection rule \eqref{eq:xue:3} has more chance to successfully detect samples as OOD. The ID conditional density $p^{hc}$ or $p^{lc}$ is small (for example, far from the HC ID samples or near the estimated LC ID samples), and we assign the OOD label to the sample because the log probability will be small enough. 

% \vspace{-0.1cm}
% \subsection{Nonparametric density estimator}\label{sec:app_density}
% \vspace{-0.1cm}
% Until now, how to estimate the local density and LC ID sample set in \eqref{eq:xue:3} remains unclear. In this subsection, we apply KNN to approximate local densities~\cite{zhao2022analysis} and derive our decision rule. In section~\ref{sec:ood_sample}  we show how to estimate the LC ID sample set. To facilitate our discussion, we first consider an artificial setting in that we know the true in/out label of the test samples, and every sample is normalized by its $l_2$ norm to project the representation onto the unit sphere. For a given test sample $x$, we first use cosine similarity to collect the $k$ closet samples from $x$ as ${D}_{KNN}(x)$ from ${D}^{in}\cup {D}^{test}$, where ${D}^{test}$ is test time sample set that follows some mixed distribution of ID/OOD. Without loss of generality, we assume ${D}_{KNN}(x)$ to contain $k_1$ and $k_2$ samples from HC/LC ID, respectively. We denote two disjoint datasets ${D}_{KNN}^{hc}(x)$ and ${D}_{KNN}^{lc}(x)$ containing the HC ID/LC ID samples in ${D}_{KNN}(x)$. Next, we make an assumption on the conditional densities $p^{hc}(x|x_i)$ and $p^{lc}(x|x_j)$ as follows:


% {\it Assumption 1:} There exist two positive constants $\lambda_{hc} <\lambda_{lc}$ such that $p^{hc}(x|x_i)$ and $p^{lc}(x|x_j)$ are proportional to $\exp(-\lambda_{hc}\|x-x_i\|_2)$ and $\exp(-\lambda_{lc}\|x-x_j\|_2)$.\footnote{Here we assume the density function's tails performance being exponential. Via more sophisticated analysis, we may further relax the density being subgaussian/subexponential.}

%  We use $\lambda_{hc}$ and $\lambda_{lc}$ to describe the influence of HC ID and LC ID samples. Let us consider a sample $x$ and a reference point $y$ that is close to $x$. 
%  Intuitively, one may expect that $x$ has a higher chance of being an ID sample if $y$ is an HC ID sample and a lower chance if $y$ is believed from LC ID sample. In other words, for the same reference sample $y$, we should have $p^{hc}(x|y)> p^{lc}(x|y)$, which is achieved by setting $\lambda_{hc}<\lambda_{lc}$ in {\it Assumption 1}. During the testing stage, we can hardly ensure $y$ is from ID or OOD distribution. Therefore it would be safer to treat  $y$ as a reference sample that contributes less than a normal ID reference sample in assessing the chance of sample $x$ being ID.\footnote{If the exact OOD sample set is available in the test stage, the OOD detection task fall into the semi-supervised learning field, and we may use the log-likelihood-ratio~\cite{kawakita2013semi} as the score function, i.e., $S(x|{D}^{in},\hat{{D}}^{out}) \propto \log \left({\mathbbm{P}(x\textrm{ from ID}|{D}^{in})}/{\mathbbm{P}(x\textrm{ from OOD}|{D}^{out})}\right) %= \log \mathbbm{P}(x\textrm{ from ID}|\mathcal{D}^{in}) - \log \mathbbm{P}(x\textrm{ from OOD}|\mathcal{D}^{out})$.} 
%  $. We detail the empirical results and comparison in section~\ref{sec:app_log}.} We then combine {\it Assumption 1} with ${D}^{hc}_{KNN}(x)$ and ${D}^{lc}_{KNN}(x)$ instead of ${D}^{hc}$ and $\hat{{D}}^{lc}$ in terms $(a)$ and $(b)$.  
% \vspace{-0.1cm}
% \begin{align}
% \tiny
% &(a)\propto - \sum_{x_i\in{D}^{hc}_{KNN}(x)}\lambda_{hc}\|x-x_i\|_2\notag \quad;\quad(b)\propto - \sum_{x_i\in{D}^{lc}_{KNN}(x)}\lambda_{lc}\|x-x_i\|_2\notag\\
% % + \sum_{x_j\in \mathcal{D}_{KNN}^{out}(x)}\lambda_{x_j}\|x-x_j\|_2\notag\\
% % \Rightarrow &S(x|\mathcal{D}^{in}_{KNN}(x),\mathcal{D}^{out}_{KNN}(x)) \propto -\sum_{x_j\in\mathcal{D}_{KNN}(x)} \|x-x_j\|_2 \cdot s(x_j),\label{eq:xue:4}
% \Rightarrow& (a) + (b) \propto -\sum_{x_i\in{D}_{KNN}(x)}\|x-x_i\|_2\cdot s_i\label{eq:xue:4}
% \end{align}
% where we set $s_j = 1$ if $x_j$ is from HC ID and $s_j = \lambda_{lc}/\lambda_{hc}$ otherwise. Finally combine \eqref{eq:xue:4} with \eqref{eq:xue:3} and we end up with the decision rule used in {\bf Algorithm~\ref{alg1:decision} line 7}:
% \vspace{-0.1cm}
% \begin{align}
% \mathbf{I}\left\{-\sum_{x_j\in{D}_{KNN}} \|x-x_j\|_2 \cdot s_j \ge \lambda\right\}\label{eq:xue:5}
% \end{align}
% \vspace{-0.1cm}
% Note that in the detection rule \eqref{eq:xue:5}, we require the knowledge on the distribution labels for all samples in ${D}_{KNN}$, which is inaccessible for samples from ${D}_{test}$ in practice. In this paper, we instead propose an estimation of distribution labels via \eqref{eq:xue:5} with a slightly larger $\lambda$. Since usually the ID sample size $N$ is much larger than the test sample size $n$, detecting extra ID samples only leads to marginal improvement. We may directly use $\mathcal{D}^{in}$ instead of all ID samples. 


% We use two scenarios in~\figurename~\ref{fig:motivation} to show the rationality of the decision rule \eqref{eq:xue:5}. 
% \begin{figure}
%     \centering
%     \includegraphics[width=0.4\textwidth]{imgs/motivation.pdf}
%     \caption{\small $\mathcal{D}^{out}=\mathcal{N}(10,1/2)$.}
%         \label{fig:motivation1}
% \end{figure}
% % \begin{wrapfigure}{r}{0.2\textwidth}
% %   \begin{center}
% %   \advance\leftskip+1mm
% %     \vspace{-0.2in}  
% %     \includegraphics[width=0.3\textwidth]{imgs/motivation.pdf}
% %     \vspace{-0.2in} 
% %     \caption{\small $\mathcal{D}^{out}=\mathcal{N}(10,1/2)$.}
% %         \label{fig:motivation1}
% %     \vspace{-0.2in} 
% %   \end{center}
% % \end{wrapfigure}

% \textit{Well separated ID/OOD in~\figurename~\ref{fig:motivation1}.} In this scenario, when $(a)$ in \eqref{eq:xue:4} is large enough (i.e., $x$ in a high-density regime of HC ID distribution), the density of LC ID distribution at $x$ must be very small, then $\log p^{lc}\approx 0$. In this case, the decision rule reduces to the classic detection rule \eqref{eq:xue:0}. On the other hand, when $x$ is from LC ID distribution, both $(a)$ and $(b)$ are expected to be small (large $\lambda_{lc}$ reduce the contribution of $p^{lc}$), and we can safely assign the OOD label while sacrificing minimal ID accuracy.

% \textit{Overlapped ID/OOD in~\figurename~\ref{fig:motivation2}.} In this setting, we consider the ID/OOD overlap in some high-density regimes. The classic OOD detection rule \eqref{eq:xue:0} has a small threshold $\lambda$ and can lead to a large number of OOD samples being classified as ID samples. When applying the detection rule \eqref{eq:xue:4}, we measure the conditional density given both HC ID/LC ID sample sets. As long as one of the terms $(a)$ or $(b)$ is small enough, which corresponds to the situations where $x$ is far from the HC ID reference samples or has enough close estimated LC ID reference samples, we can still assign the sample $x$ with the OOD label. Our method, hence, yields a lower false positive rate.


% \subsubsection{Estimation of OOD sample set.}\label{sec:ood_sample}
% Next, we consider the estimation of the OOD sample set. Let denote ${D}_{KNN}^{lc,T}$ and ${D}_{KNN}^{lc,F}$ as the disjoint sample sets containing the true OOD sample and false OOD sample in ${D}_{KNN}^{lc}$. We will have the following separation:
% \begin{align}
% \tiny
% -\sum_{x_j\in{D}_{KNN}} s(x_j)\|x-x_j\|_2=
% -\sum_{x_j\in{D}_{KNN}^{lc,T}(x)}s(x_j)\|x-x_j\|_2 
% -\sum_{x_j\in{D}_{KNN}^{lc,F}(x)}s(x_j)\|x-x_j\|_2.  
% \end{align}
% If we overestimated the OOD sample size by a margin, the corresponding $\sum_{x_j\in {D}_{KNN}^{lc}(x)}\|x-x_j\|_2s(x_j)$ will be overestimated and yield a lower AUC on ID/OOD detection. On the other hand, if we only collect the LC ID sample with enough confidence (e.g., the small enough value from the score function), the corresponding $\sum_{x_j\in {D}_{KNN}^{lc}(x)}\|x-x_j\|_2s(x_j)$ becomes smaller and the decision rule of \eqref{eq:xue:5} leans more on the high confidence ID samples. In the extreme case, the ${D}_{KNN}^{lc}(x)$ being empty set, the $\sum_{x_j\in {D}_{KNN}^{lc}(x)}\|x-x_j\|_2s(x_j)$ becomes 0 and the detection rule \eqref{eq:xue:5} reduces to the classic detection rule \eqref{eq:xue:0}. Therefore, only keeping the test sample with high confidence, as the detected OOD sample is safer. In this paper, we propose to use the following decision rule to collect the estimated OOD samples during the test stage ({\bf Algorithm~\ref{alg1:decision} line 9}):
% \begin{align}
% \mathbf{I}\left\{S(x_0|{D}^{hc}_{KNN}(x),\hat{{D}}^{lc}_{KNN}(x))<\lambda\cdot \gamma\right\},
% \end{align}
% where $\gamma\ge 1$ and $\hat{{D}}^{lc}_{KNN}(x)$ is the estimated OOD sample set and is empty at the beginning.



% \section{Why shouldn't we use the log ratio test?}\label{sec:app_log}

% As illustrated in Section~\ref{sec:app_density}, If the exact OOD sample set is available in the test stage, the OOD detection task falls into the semi-supervised learning field, and we should use the log-likelihood-ratio~\cite{kawakita2013semi} as the score function, i.e., $S(x|{D}^{in},\hat{{D}}^{out}) \propto \log \left({\mathbbm{P}(x\textrm{ from ID}|{D}^{in})}/{\mathbbm{P}(x\textrm{ from OOD}|{D}^{out})}\right)$. Consequently, the final score function will be 

% \begin{equation}
%   S(x_o)=\frac{1}{k}\sum_{i=1}^k \mathbf{1}\{y_i=OOD\}\parallel z_o-z_{(i)} \parallel s_{(i)}-\frac{1}{k}\sum_{i=1}^k \mathbf{1}\{y_i=ID\}\parallel z_o-z_{(i)} \parallel s_{(i)}  \label{equ:log_ratio}
% \end{equation}


% As depicted in Table.~\ref{tab:log_ratio}, we observed notable OOD detection performance when a subset of OOD samples was accessible prior to the test phase. In our experiments, we preselected $10\%$ of the test set as OOD samples for log-ratio score calculation using \eqref{equ:log_ratio}. However, practical scenarios rarely offer the luxury of pre-access to OOD samples. In these cases, we adopt a strategy where each test sample is evaluated, and those with low confidence are stored as an estimated OOD distribution. This approach encounters challenges, primarily stemming from two factors:

% 1. \textbf{The Cold Start Problem}: At the outset of the test, the set of low-confidence samples is empty, leading to highly unstable and unreliable scores calculated in the early stages.

% 2. \textbf{Inaccurate Estimation}: As previously mentioned, it's impossible to guarantee that every sample in the low confidence set is genuinely an OOD sample. This introduces noise into the data, making \eqref{equ:log_ratio} susceptible to inaccuracies.

% In contrast, our proposed method, referred to as \abbr, effectively addresses these issues.





% \section{Additional Experimental Results}\label{sec:addexp}

% \subsection{Additional ablation studies}
